# Supplementary material for: Overcoming the rate-distance barrier of quantum key distribution without using quantum repeaters
Source: arXiv:1811.06826 ancillary file (2018-11-16)
Supplement: Supplementary file 1 [file TF-QKD_supplementary.pdf]

# Supplementary Information

## “Overcoming the rate-distance barrier of quantum key distribution without using quantum repeaters”

## Fibre-based experiments

All the experiments represented in Fig. 1a are numbered in chronological order. The correspondence between numbers and references (following in square brackets) is: 1 → [31]; 2 → [32]; 3 → [33]; 4 → [34]; 5 → [35]; 6 → [36]; 7 → [37]; 8 → [38]; 9 → [3]; 10 → [39]; 11 → [40]; 12 → [41]; 13 → [42]; 14 → [4]; 15 → [43]; 16 → [44].

## Protocol

0. *Initial operations* – The phase interval $[0, 2\pi)$ is split into $M = 16$ equal slices $\Delta_k = 2\pi k/M$, with $k = \{0, ..., M-1\}$. An authenticated channel is set up for the public announcements made by the legitimate users Alice and Bob.
1. *Classical stage* – The users send bright unmodulated optical pulses to the relay station, to let Charlie stabilise the communication channels and in particular minimise the phase misalignment $\delta_{ba} = \delta_b - \delta_a$.
2. *Quantum stage* – The users attenuate the optical pulses to the single-photon level and modulate their phase and intensity.
3. *Preparation* – Alice and Bob select random values for the intensities $\mu_{a,b} \in \{u/2, v/2, w/2\}$; the bit phases $\alpha_{a,b} \in \{0, \pi\}$, corresponding to the bits $\{0, 1\}$, respectively; the basis phases $\beta_{a,b} \in \{0, \pi/2\}$, corresponding to the bases $\{X, Y\}$, respectively; and the phases $\rho_{a,b} \in [0, 2\pi)$. They record in which phase slice $\Delta_{k(a)}$ (Alice) or $\Delta_{k(b)}$ (Bob) their values $\rho_a$ and $\rho_b$ fall into. They then prepare pulses with intensities $\mu_{a,b}$ and phases $\varphi_{a,b} = (\alpha_{a,b} + \beta_{a,b} + \rho_{a,b}) \oplus 2\pi$ and send them to Charlie.
4. *Charlie's measurement and announcement* – Charlie interferes the incoming pulses and records which detector clicks. When the quantum communication is over, he publicly announces all the runs where his detector 0 (1) clicked; Alice and Bob will correspondingly set a variable $\chi$ equal to 0 ($\pi$). All the runs where none of or both of his detectors clicked are discarded.
5. *Users's announcement and sifting* – After the previous step is complete, Alice announces the intensities $\mu_a$, the basis phases $\beta_a$ and the phase slices $\Delta_{k(a)}$ and Bob announces the runs where his values match Alice's. The users discard all the mismatched runs. Then they disclose the bit values of the matched runs except those in basis $X$ and intensity class $u$, which are kept secret.
6. *Raw key bit distillation and parameter estimation* – The users perform a coordinated random permutation of the bits. For the bits in basis $X$ and intensity class $u$, Bob draws Alice's bit phase $\alpha_a$ from the relation $\chi = |\alpha_b - \alpha_a|$. The users can then distill a key bit equal to 0 (1) when $\alpha_a = 0$ ($\pi$). A raw key is formed by concatenating these bits. All the remaining bits, fully disclosed in the previous step, are used to perform the decoy-state parameter estimation and test the channel against the presence of Eve.
7. *Post-processing* – The users run classical post-processing procedures such as error correction and privacy amplification to distil the final secure key from the raw key.

**Table S1 – TF-QKD protocol**.

In Table S1 we list the steps of the TF-QKD protocol. For definiteness, we specialise it to the case with $M = 16$ and we consider the realistic setting where the decoy-state technique is implemented with three

levels of intensity. The generalisation to a different number of phase slices or of intensity settings is straightforward.

We use the symbol "$\oplus 2\pi$" for "addition modulo $2\pi$", which is used to map a generic phase value to the interval $[0, 2\pi)$. As in the rest of the paper, we use the compressed subscript notation $x_{a,b}$ to indicate $x_a, x_b$, the first label referring to Alice and the second to Bob. Following Fig. 1b, we denote $\delta_a$ and $\delta_b$ the noise variables associated with a phase misalignment of Alice's and Bob's optical pulses when interfering on Charlie's beam splitter. Misalignment might be due to the different emission spectra of the lasers or to the propagation of the pulses through different fibres. All the public communications effected by the users are assumed to be authenticated.

# Active feedback

From Eq. (4) in the main text and from the TF-QKD protocol given in Table S1, we describe the phase drift due to the channels' length fluctuation as $\delta_{ba} = \delta_b - \delta_a = 2\pi\nu\Delta L/s$. To compensate this phase drift, Charlie can use an active feedback routine based on the bright pulses received by Alice and Bob during the classical stage (step 1 of the TF-QKD protocol). The reference bright pulses are unmodulated, so Charlie can act on his phase modulator (PM in Fig. 1b) until he minimises (maximises) the counts in his detector 0 (1). The bright pulses can be time-multiplexed with the quantum signals in bursts, to avoid the detrimental effect of the Raman scattering. For simplicity, we assume a duty cycle between quantum and classical optical pulses equal to $d = 50\%$, which is the value adopted in the numerical simulations. The compensation mechanism would never be perfect and any amount of uncompensated phase drift $\delta_{ba}$ would increase the channel optical error rate $e_{opt} = \sin^2(\delta_{ba}/2)$. In the numerical simulation of Fig. 1a we assumed $e_{opt} = 3\%$, which holds if $\delta_{ba} \leq 0.35$ rad. The worst-case phase drift rate is obtained for the longest-distance configuration (550 km of standard optical fibre) and amounts to 6.0 rad/ms. This is equal to 0.3 rad per 50 $\mu$s, showing that a feedback every $\sim 50$ $\mu$s would suffice to compensate the phase drift. With a clock rate of 1 GHz, a total $5 \times 10^4$ reference pulses can be distributed in this amount of time. The intensity of these reference pulses can be chosen such that they produce about 1,000 counts in Charlie's detectors, which is enough to estimate the phase drift angle and correct it using a fast actuator on Charlie's phase modulator.

# Numerical simulations

For all the simulated rates we set the clock rate equal to 1 GHz. The theoretical curves $a - d$ in Fig. 1a have been labelled starting from the lowest key rate-vs-distance figure. To draw these curves, we have set $\eta = 10^{-\alpha L/10}$, with $\alpha = 0.2$ dB/km the linear attenuation of a standard optical fibre and $L$ the distance. These curves and the one pertaining to the ideal TF-QKD have been obtained under ideal conditions, i.e., with zero detector and channel noise, maximum detection efficiency ($\eta_{det} = 100\%$) and unitary error correction efficiency ($f = 1$). The explicit key rate equations used to draw the lines in Fig. 1a are:

- *Single-repeater bound*[16] (solid line on top): $R_{\text{1rep}} = -\log_2(1 - \sqrt{\eta})$.
- *Secret key capacity*[9] (line $d$): $R_{\text{SKC}} = -\log_2(1 - \eta)$. This expression improves the previous upper bound[8] $R_{\text{SKC}} \leq -\log_2[(1 - \eta)/(1 + \eta)]$, closing the gap with the best-known lower bound,[45] and is a strong converse rate.[46]
- *Single-photon QKD* (line $c$): $R_{\text{spQKD}} = \eta$. Starting from the Shor-Preskill key rate for the BB84 protocol,[47] we set the QBER equal to zero and consider the efficient BB84 protocol,[26] which has a basis sifting factor asymptotically equal to 1.
- *Decoy-state QKD* (line $b$): $R_{\text{dsQKD}} = \eta/e$, with $e$ the Euler's number. Starting from the asymptotic key rate of the BB84 protocol with infinite decoy states,[22] we set the QBER as in the previous case and consider the efficient BB84 protocol.[26] Hence the key rate coincides with the single-photon gain $Q_1 = \eta\,(\mu e^{-\mu})$. The term in brackets is the Poisson probability that a coherent state with intensity $\mu$ contains 1 photon, which is maximised by $\mu = 1$.

- *Decoy-state MDI-QKD* (line $a$): $R_{\mathrm{dsMDI}} = \eta/(2e^2)$. Starting from the decoy-state MDI-QKD rate equation,[23] we set the QBER equal to zero and consider an efficient version of MDI-QKD, where the basis sifting factor is $\approx 1$. Then the rate coincides with the double-single-photon gain $Q_{11} = \eta_a \eta_b \left(\mu_a e^{-\mu_a} \mu_b e^{-\mu_b}\right)/2$ (see also, e.g., Ref. [48]). The term in brackets is the multiplication of two independent Poisson probabilities for the emission of 1 photon, maximised by $\mu_a = \mu_b = 1$, and the channel transmittances are $\eta_a = \eta_b = \sqrt{\eta}$, because Charlie is placed midway between Alice and Bob. This provides the rate equation given above. We notice here that we could obtain by similar reasoning the key rate of the ideal single-photon MDI-QKD, which is $R_{\mathrm{spMDI}} = \eta/2$. This is not plotted in Fig. 1a. However, the corresponding curve could easily be drawn from the one for the ideal single-photon QKD as $R_{\mathrm{spMDI}} = R_{\mathrm{spQKD}}/2$.
- *Ideal TF-QKD* (thick dashed line). For the simulations of TF-QKD, we exploit the fact that the detection scheme is the same as in ordinary QKD. It consists of single-photon interference followed by single-photon detection. This makes it possible to use the same equations as in decoy-state QKD,[22,49] under the assumptions in the security argument (see next section). Simulation-wise, it is customary and reasonable to assume that there is no eavesdropping on the line, so that only the natural noise and loss of the scheme play a role. Hence, on one hand, we consider two identical threshold detectors in Charlie's station, with the same detection efficiency. This entails that the total detected power is independent of the relative phase of the interfering beams.[50] We can then express the overall $n$-photon yield of TF-QKD as in decoy-state QKD. On the other hand, the photons populating the twin fields follow the Poisson statistics $p_{n|\mu}$ (see Eq. (2) and related discussion) and this allows us to model the gain of TF-QKD as in decoy-state QKD. We incidentally notice that this argument would not apply to decoy-state MDI-QKD,[24,46] where the users owns two independent phase-randomised photon sources and the signal depends on the coincidence counts, not on the single counts, of Charlie's detectors.

  The simulation of the ideal TF-QKD is based on Eqs. (1)–(3) of the main text, in which we replace the ideal parameters given in the inset of Fig. 1a. We set $d = 1$ and $M = 16$, which entails, from Eq. (1), $E_M = 1.275\%$. For the decoy-state estimation, we assume an infinite amount of intensity settings, as in Ref. [22]. The key bits are distilled from the pulses in the $X$-basis having total intensity $\mu = u$. The probability to prepare these pulses is asymptotically close to 1. Alice and Bob's joint single-photon quantities are $\underline{y}_1 = \hat{\eta}$, $\underline{Q}_1 = u e^{-u} \underline{y}_1$ and $\overline{e}_1 = E_M$, with $\hat{\eta} = 10^{-\frac{\alpha L/2}{10}} = \sqrt{\eta}$. Here, it is important to notice the factor $L/2$ in $\hat{\eta}$, which descends directly from Eq. (3) (see also Fig. 2) and is due to Charlie being placed midway between Alice and Bob. To simulate gain and error rate, we exploit the argument outlined above and specialise to TF-QKD the model developed for decoy-state QKD in Ref. [51]. In the limit of long distance, we have $Q_u = u\hat{\eta}$ and $E_u = E_M$. The ideal TF-QKD key rate in Eq. (3) then simplifies to $R^{(\neg\rho,\mathrm{ideal})}_{\text{TF-QKD}} = u\hat{\eta}/M\{e^{-u}\left[1 - h\left(E_M\right)\right] - h\left(E_M\right)\}$. This key rate is numerically maximised by the optimal value $u_{\mathrm{opt}} = 0.765$.
- *Realistic TF-QKD* (thick solid line). The simulation is again based on the similarity between TF-QKD and decoy-state QKD, outlined in the previous point, and on Eq. (3). We still set $M = 16$, as this value maximises the darker pink-shaded area in Fig. 1a, but this time we adopt a duty cycle coefficient equal to $d = 0.5$ and the realistic parameters reported in the bottom row of the inset of Fig. 1a. For the decoy state estimation, Alice and Bob use three intensity settings $\mu_{a,b} \in \{w/2, v/2, u/2\}$, with $w = 10^{-4}$, $v = 10^{-2}$ and $u = 0.4$, prepared with probabilities $p_w = p_v \ll p_u = 1 - p_v - p_w \lesssim 1$. We associate the signals with the intensity $u$. According to the TF-QKD protocol, the key bits are distilled only from this intensity class. Alice and Bob's joint single-photon quantities are[49] $\underline{y}_1 = \left[u^2 Q_v e^v - u^2 Q_w e^w - (v^2 - w^2)\left(Q_u e^u - \underline{y}_0\right)\right] / \left[u(uv - uw - v^2 + w^2)\right]$ and $\overline{e}_1 = (E_v Q_v e^v - E_w Q_w e^w)/\left[(v - w)\underline{y}_1\right]$, where $\underline{y}_0 = (vQ_w e^w - wQ_v e^v)/(v - w)$. For gain and error rate, we start again from the model in [51]. We find $Q_u = 1 - (1 - P_{dc})^2 e^{-u\tilde{\eta}}$, with $\tilde{\eta} = \eta_{det} \times \hat{\eta}$, $\eta_{det} = 30\%$ and $P_{dc} = 10^{-8}$ the dark count probability per gate for a detector clocked at 1 GHz. This parameter has equivalently been expressed in Hz in the inset of Fig. 1a. The gains $Q_v$, $Q_w$ are analogous to $Q_u$ and can be obtained by replacing $u$ with $v$ or $w$, respectively. For the error rates, $E_u = 1/2 + 1/(2Q_u)(1 - P_{dc})\{e^{-u\tilde{\eta}[1-(e_{opt}+E_M)]} - e^{-u\tilde{\eta}(e_{opt}+E_M)}\}$, with $e_{opt} = 3\%$. The error rates $E_v$, $E_w$

are analogous to $E_u$. Nearly identical results have been obtained replacing the above analytical decoy state estimation with an equivalent numerical formulation.

# Security argument

In this section, we justify the key rate reported in Eq. (3) of the main text. Our approach is in three steps. First, we will reduce TF-QKD to a scheme that is analogous to the well-known BB84 protocol.[1] This will allow us to borrow some of the mathematical tools already developed for this protocol. As a second step, we will study the security of the BB84-like scheme assuming a perfect single-photon source. Lastly, we will extend the security from the single-photon setup to a more practical light source that emits weak coherent pulses. This part contains the main open challenge to determine the ultimate key rate of TF-QKD when Eve makes use of the global phase information disclosed in the TF-QKD protocol's step 5.

To emphasize the security-oriented cut of this section, we replace the user "Charlie" appearing in the main text with the eavesdropper "Eve". This replacement can only make the security analysis stronger, as Eve is given full access to Charlie's equipment. In the TF-QKD protocol, Eve can decide to not cooperate with Alice and Bob, e.g., by not performing any measurement, or by not disclosing the (correct) results. This would represent a denial-of-service attack, which is always possible in QKD. However, if Eve decides to cooperate, she cannot cheat and either Alice and Bob successfully distil a secure key or they abort the key distillation protocol.

In the security argument, we assume that ideal faultless equipment is used and that the legitimate users strictly adhere to the protocol. All the light signals are assumed to be single mode and, in particular, in the same polarisation state. We exclude any leakage of side information from the setup due to an imperfect implementation of the protocol, either accidentally caused by the users or purposely triggered by Eve. Finally, we work in the asymptotic regime and neglect the detrimental effect due to the finiteness of the experimental data sample.

## Notation

Let us start by introducing the notation. As already mentioned, we use the compressed subscript notation $x_{a,b}$ to indicate $x_a, x_b$, the first label referring to Alice and the second to Bob. We define the photon-number states (Fock states) as in the main text, denoting $|n\rangle$ the Fock state containing $n$ photons. A coherent state with intensity $\mu$ and electromagnetic phase $\theta$ is then written as $|e^{i\theta}\sqrt{\mu}\rangle = e^{-\frac{\mu}{2}} \sum_{n=0}^{\infty} e^{in\theta} \mu^{\frac{n}{2}} / \sqrt{n!} |n\rangle$, with $i$ the imaginary unit. It is also convenient for later use to define the single-photon entangled states,

$$|\psi^{\pm}\rangle_{ab} = \left(|0\rangle_a |1\rangle_b \pm |1\rangle_a |0\rangle_b\right) / \sqrt{2}, \tag{S1}$$

and the phase operator $\hat{U}^{(\theta)}$,

$$\hat{U}^{(\theta)}_{a,b} |0\rangle_{a,b} = |0\rangle_{a,b}, \tag{S2}$$

$$\hat{U}^{(\theta)}_{a,b} |1\rangle_{a,b} = e^{i\theta} |1\rangle_{a,b}. \tag{S3}$$

We now introduce some auxiliary single-photon states. We define the $Z$-basis eigenvectors as $|z_+\rangle = \left(\begin{smallmatrix}1\\0\end{smallmatrix}\right)$, $|z_-\rangle = \left(\begin{smallmatrix}0\\1\end{smallmatrix}\right)$, and the $X$-basis and $Y$-basis eigenvectors as $|x_\pm\rangle = (|z_+\rangle \pm |z_-\rangle)/\sqrt{2}$ and $|y_\pm\rangle = (|z_+\rangle \pm i|z_-\rangle)/\sqrt{2}$, respectively. $I = \left(\begin{smallmatrix}1&0\\0&1\end{smallmatrix}\right)$ will be the bidimensional identity matrix and $X = \left(\begin{smallmatrix}0&1\\1&0\end{smallmatrix}\right)$, $Y = \left(\begin{smallmatrix}0&-i\\i&0\end{smallmatrix}\right)$, $Z = \left(\begin{smallmatrix}1&0\\0&-1\end{smallmatrix}\right)$ will be the three Pauli matrices. We write the two-photon maximally entangled states (Bell

states) in the various bases as:

$$|\Psi_Z^{\pm}\rangle_{ab} = \left(|z_+\rangle_a |z_-\rangle_b \pm |z_-\rangle_a |z_+\rangle_b\right)/\sqrt{2}, \tag{S4}$$

$$|\Phi_Z^{\pm}\rangle_{ab} = \left(|z_+\rangle_a |z_+\rangle_b \pm |z_-\rangle_a |z_-\rangle_b\right)/\sqrt{2}, \tag{S5}$$

$$|\Psi_X^{\pm}\rangle_{ab} = \left(|x_+\rangle_a |x_-\rangle_b \pm |x_-\rangle_a |x_+\rangle_b\right)/\sqrt{2}, \tag{S6}$$

$$|\Phi_X^{\pm}\rangle_{ab} = \left(|x_+\rangle_a |x_+\rangle_b \pm |x_-\rangle_a |x_-\rangle_b\right)/\sqrt{2}, \tag{S7}$$

$$|\Psi_Y^{\pm}\rangle_{ab} = \left(|y_+\rangle_a |y_-\rangle_b \pm |y_-\rangle_a |y_+\rangle_b\right)/\sqrt{2}, \tag{S8}$$

$$|\Phi_Y^{\pm}\rangle_{ab} = \left(|y_+\rangle_a |y_+\rangle_b \pm |y_-\rangle_a |y_-\rangle_b\right)/\sqrt{2}. \tag{S9}$$

In the discussion, we will also use the following relations between some of the Bell states,

$$|\Psi_Y^{-}\rangle_{ab} = i|\Psi_X^{-}\rangle_{ab}, \tag{S10}$$

$$|\Phi_Y^{-}\rangle_{ab} = i|\Phi_X^{-}\rangle_{ab}, \tag{S11}$$

which are easily verifiable using the definition of $|z_\pm\rangle$, $|x_\pm\rangle$ and $|y_\pm\rangle$ given above.

## Reduction to a BB84-like scheme

Target of this section is to reduce TF-QKD to another scheme that is easier to analyse and equally secure or less secure than TF-QKD. This way, the security of the weaker scheme will automatically imply the security of TF-QKD. We will achieve the target by gradually modifying some features in the physical layout of the scheme or in its classical communication part.

As a first step, we consider the TF-QKD scheme in Fig. 2c of the main text. Its main security feature is that each transmitter is inaccessible to the eavesdropper (grey-shaded areas). Therefore we can redraw this setup as in Fig. S1a, i.e., with a single area inaccessible to Eve that includes two distinct transmitters. We assume that these transmitters are perfectly locked to each other. This is the same assumption used for phase-based MDI-QKD[18] and is not restrictive. To see that, we analyse the states of the emitted optical pulses.

The laser on path $a_1$ emits pulses with intensity $\mu_a$ in a coherent state $|\sqrt{\mu_a}\rangle$. Similar states, but with intensity $\mu_b$, are emitted by the laser on path $b_1$. If the states are perfectly locked, there is no phase difference between the two lasers, so that the resulting joint state can be written without loss of generality as $|\sqrt{\mu_a}\rangle_{a_1}|\sqrt{\mu_b}\rangle_{b_1}$. On the other hand, if the lasers are imperfectly locked, we could write the joint state as $|\sqrt{\mu_a}\rangle_{a_1}|e^{i\delta_{ba}^{\rm lock}}\sqrt{\mu_b}\rangle_{b_1}$ (points 1 in Fig. S1a), where $\delta_{ba}^{\rm lock}$ is the phase difference due to the imperfect locking (dashed box in the figure), counted from Alice's phase. After the encoding with the random phases $\rho_{a,b}$ and the random bit and basis values $\gamma_{a,b}$ (points 2 and 3, respectively, in Fig. S1a), the state emitted by perfectly locked lasers would be

$$|e^{i\gamma_a}e^{i\rho_a}\sqrt{\mu_a}\rangle_{a_1}|e^{i\gamma_b}e^{i\rho_b}\sqrt{\mu_b}\rangle_{b_1}, \tag{S12}$$

whereas the one associated with imperfectly locked lasers would be

$$|e^{i\gamma_a}e^{i\rho_a}\sqrt{\mu_a}\rangle_{a_1}|e^{i\gamma_b}e^{i\rho_b}e^{i\delta_{ba}^{\rm lock}}\sqrt{\mu_b}\rangle_{b_1}. \tag{S13}$$

However, because the phase encoding operations in Fig. S1a commute, this latter state could equally have been obtained starting with the state emitted by two perfectly locked lasers, Eq. (S12), and then letting Eve encode the phase $\delta_{ba}^{\rm lock}$ herself after the pulses emerge from the protected area (point 3 in the figure).

Let us note that the commuting property between the phase encoding operations of $\delta_{ba}^{\rm lock}$ and $\gamma_{a,b}$ cannot be given as granted. Security-wise, it means that the noise related to imperfect phase-locking is independent of the bases chosen by the users. In fact, suppose that Eve wanted to add (basis-dependent) noise only to one of the states prepared by the users, for instance the one with $\gamma_{a,b} = 3\pi/2$. For that, she should wait until Alice and Bob encode their states and then add her noise, conditional on the

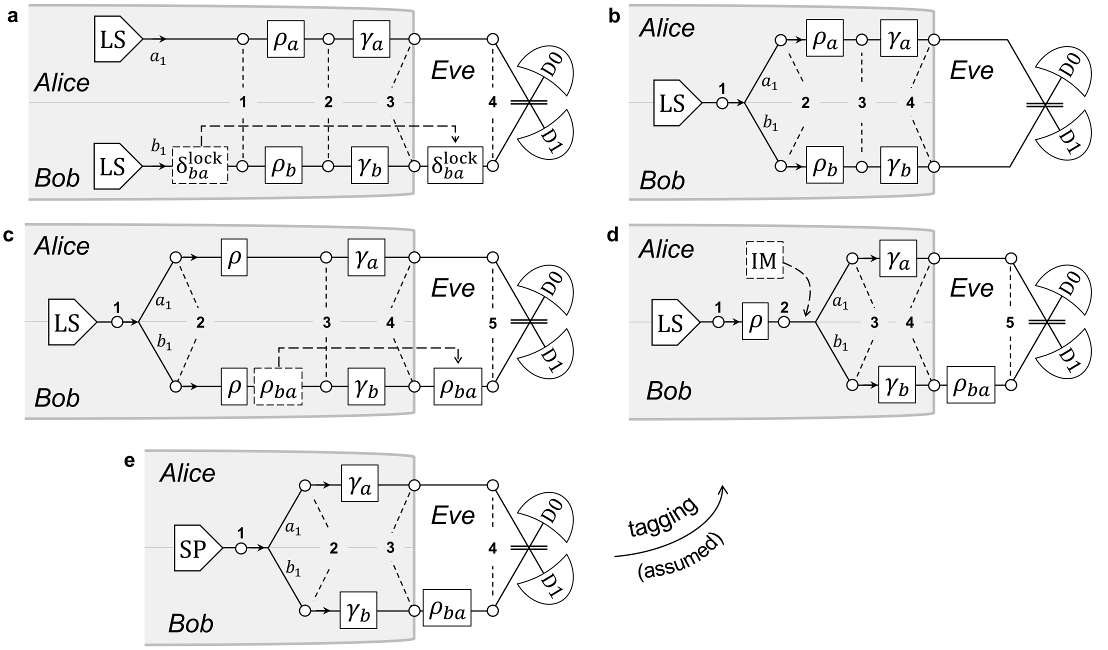


Figure S1: **Transmitters used for the reduction argument of TF-QKD.** The grey-shaded areas are inaccessible to Eve. The numbered points are for easy referencing from the text. LS: laser source; SP: single-photon source.

states chosen by the users. In this case, the time sequence of the operations is important to Eve and swapping the encoding operations is not legitimate. The described attack could be triggered, e.g., by an imperfect phase modulator, which often introduces an offset in only one of the encoded states. In this case, because the noise is basis-dependent, the commuting property of the phase encoding operations fails and the analysis has to be modified.[52] However, we assumed ideal components. Moreover, the phase locking mechanism is independent of the basis. Therefore we are allowed to swap it with the other phase operators in the preparation stage.

We also note that this form of basis-independent noise is similar to the one in the "unbalanced BB84".[53] Because the noise affects equally all the encoded states, it does not represent a security risk and it only changes the experimental data.[54,55]

Since the noise $\delta_{ba}^{\text{lock}}$ deriving from imperfect locking only entails a noisier communication and does not impact the security of the scheme, we will omit it henceforth.

Similarly to the phase-locking noise, other physical differences between the users' lasers (frequency, polarization, temporal shape, etcetera) do not affect the security of the scheme, provided that they do not leak side information to Eve, which is excluded by our assumptions. So we can consider, without loss of generality, the case where the two lasers in Fig. S1a are identical in all degrees of freedom and perfectly locked.

From here, we can go to the scheme in Fig. S1b and imagine that the users share the same laser rather than two identical lasers. In fact, the resulting scheme emits quantum states that are indistinguishable from those in Fig. S1a. The single laser in Fig. S1b emits a pulse in the coherent state $|\sqrt{\mu}\rangle$ (point 1), which impinges on a beam splitter and emerges as two pulses on paths $a_1$ and $b_1$ with intensity $\mu_a$ and $\mu_b$, respectively, with $\mu = \mu_a + \mu_b$ (point 2). The secondary pulses are encoded with phases $\rho_{a,b}$ and $\gamma_{a,b}$ and are launched into the quantum channel. The joint Alice-Bob state seen by Eve (point 4) is then $|e^{i\gamma_a}e^{i\rho_a}\sqrt{\mu_a}\rangle_{a_1}|e^{i\gamma_b}e^{i\rho_b}\sqrt{\mu_b}\rangle_{b_1}$, which coincides with the one in Eq. (S12).

To move from Fig. S1b to Fig. S1c, we equalise the random phases $\rho_{a,b}$. This is a crucial step and deserves some attention. To equalise $\rho_a$ and $\rho_b$, the users need to declare their random phases on the

public channel and discard all the runs where the phases do not exactly match. For the moment, we assume that this operation does not affect the security of the protocol. We will discuss later on the implications of this assumption. Our target here is limited to showing that the classical information given to Eve in the scheme of Fig. S1c is larger than or equal to the one disclosed in TF-QKD.

In TF-QKD, only the phase slices $\Delta_{k(a,b)}$, not the exact phase values $\rho_{a,b}$, are disclosed (step 5 of the protocol). Announcing $\rho_{a,b}$ can only give more information to Eve than announcing $\Delta_{k(a,b)}$, so it is not restrictive to assume that in the scheme of Fig. S1b Alice and Bob announce the complete $\rho_{a,b}$. Then, we can set without loss of generality $\rho_a = \rho$ and $\rho_b = \rho + \rho_{ba}$, so to rewrite the resulting output state as

$$|e^{i\gamma_a} e^{i\rho} \sqrt{\mu_a}\rangle_{a_1} |e^{i\gamma_b} e^{i\rho} e^{i\rho_{ba}} \sqrt{\mu_b}\rangle_{b_1}. \tag{S14}$$

This is the output state of the transmitter in Fig. S1c. In the associated protocol, Alice will announce $\rho$ and Bob will announce $\rho_{ba}$ so that the total disclosed information is equal to the previous scheme. Notice that Bob can calculate $\rho_{ba}$ after learning $\rho$ from Alice, and this is in accordance with the TF-QKD protocol's step 5, where Alice announces first and Bob second.

Security-wise, it is crucial that Eve does not learn the value of the global random phase $\rho$ before the users disclose it in the step 5 of the protocol. However, the relative random phase $\rho_{ba}$ is different and can be given to Eve. Proving security without relying on $\rho_{ba}$ would automatically entail the security of the previous schemes, where $\rho_{ba}$ is revealed during the protocol's step 5.

So we swap the encoding operations for $\rho$, $\rho_{ba}$ and $\gamma_a$ (they all commute, so this will not alter the outcomes) and assign $\rho_{ba}$ to the quantum channel, as if it were encoded directly by Eve. This explicitly shows that we will not use $\rho_{ba}$ to prove security. In fact, we could even omit this variable from the discussion. However, because $\rho_{ba}$ is part of the announcement stage and it also represents unavoidable phase noise in TF-QKD, we will carry it on as a variable fully known to Eve.

The last step in the reduction argument is presented in Fig. S1d, where the random secret phase $\rho$ is encoded *before* the splitting point into paths $a_1$ and $b_1$. It is easy to see that the output state at point 4 in Fig. S1d coincides with the output state at point 4 in Fig. S1c. Omitting the variable $\rho_{ab}$, which has been assigned to Eve, the output state reads

$$|e^{i\gamma_a} e^{i\rho} \sqrt{\mu_a}\rangle_{a_1} |e^{i\gamma_b} e^{i\rho} \sqrt{\mu_b}\rangle_{b_1}. \tag{S15}$$

To obtain this state, it suffices to specify the beam splitter's reflection as $R = \mu_a/\mu$ (transmission as $T = \mu_b/\mu$), where $\mu = \mu_a + \mu_b$, and apply the usual input-output relations of the beam splitter to the input state $|e^{i\rho}\sqrt{\mu}\rangle|0\rangle$.

The scheme in Fig. S1d resembles the transmitter of a phase-based BB84 protocol implemented with phase-randomised weak coherent pulses and emits exactly the same states, given by Eq. (S15). The random phase $\rho$ takes values in $[0, 2\pi)$ and the encoding phases $\gamma_{a,b}$ generate a relative phase $\gamma_{ba} = (\gamma_b - \gamma_a) \oplus 2\pi$ between the two time bins on paths $a_1$ and $b_1$ that takes values in $\{0, \pi/2, \pi, 3\pi/2\}$, as in the phase-encoded BB84. Moreover, by inserting the intensity modulator (IM) in the setup of Fig. S1d, the transmitter becomes equivalent to the typical transmitter used to implement the phase-based decoy-state BB84 protocol. The IM can be equivalently described as two independent IMs placed on paths $a_1$ and $b_1$, as in the TF-QKD scheme in Fig. 1b of the main text, provided that the users post-select only equal intensity classes during the public discussion, which is prescribed by the TF-QKD protocol's step 5. This does not automatically imply that we can use decoy states in TF-QKD, which still has to be proven.

Despite the similarity with the BB84 protocol, the scheme in Fig. S1d is not equivalent to it. The most apparent difference is that in BB84 the emitted signals are analysed by a trusted receiver, whereas in the scheme in Fig. S1d they are measured by Eve herself. A second difference is that the value of the random phase $\rho$ is announced in the scheme of Fig. S1d whereas it is not announced in the BB84 protocol. Therefore we cannot yet conclude that this scheme is as secure as the BB84 protocol.

However, we will show that the structure of the security proof is the same as the BB84 protocol's one, so we can adapt it to the new scheme. With this in mind, we will first analyse the case of a perfect single-photon source, given in Fig. S1e, to then extend the result to the more practical source used in

Fig. S1d. By virtue of the reduction argument, the security of TF-QKD will then follow from the one of the scheme in Fig. S1d.

## Single-photon source (Fig. S1e)

In this section, we analyse the security of the scheme in Fig. S1e, which is the same as in Fig. S1d, but with the light source and the phase randomiser replaced by a perfect single-photon source. To prove its security, we will follow the structure of BB84 protocol's security proofs.[47,56,57] We will show that the users can distill entanglement at distance using a shared single photon inaccessible to Eve. Then we will study the protocol in the $X$ basis and derive its bit-error and phase-error rates. Finally, we will show that the phase-error rate can be estimated from the bit-error rate in the $Y$ basis.

In the scheme of Fig. S1e, the single-photon source emits a photon number state $|1\rangle$ (point 1 in the figure), which is then split in the two paths $a_1$ and $b_1$ by a beam splitter that we assume, for simplicity, to be 50:50. This implies $\mu_a = \mu_b$ in the original protocol, which is guaranteed by the protocol's sifting procedure. The state at point 2 in Fig. S1e is then given by $|\psi^+\rangle_{a_1 b_1} = \left(|0\rangle_{a_1}|1\rangle_{b_1} + |1\rangle_{a_1}|0\rangle_{b_1}\right)/\sqrt{2}$, see Eq. (S1).

In TF-QKD, the encoding variables are $\gamma_{a,b}$. The output states of the setup in Fig. S1e (point 3) can then be obtained by applying the phase operators $\hat{U}^{(\gamma_{a,b})}_{a_1,b_1}$ to the initial state $|\psi^+\rangle_{a_1 b_1}$. Up to an inessential global phase, we obtain:

$$\hat{U}^{(\gamma_b)}_{b_1}\hat{U}^{(\gamma_a)}_{a_1}|\psi^+\rangle_{a_1 b_1} = \frac{e^{i(\gamma_b-\gamma_a)}|0\rangle_{a_1}|1\rangle_{b_1} + |1\rangle_{a_1}|0\rangle_{b_1}}{\sqrt{2}}. \tag{S16}$$

The values of $\gamma_{a,b}$ are given by the sum of the bit phases, $\alpha_{a,b} = \{0, \pi\}$, and the basis phases, $\beta_{a,b} = \{0, \pi/2\}$, and the $X$ and $Y$ bases are associated with $\beta_{a,b} = 0$ and $\beta_{a,b} = \pi/2$, respectively. By convention we set $X$ as the *computational* basis, from which key bits are distilled, and $Y$ as the *test* basis, from which the potential presence of Eve is detected.

If the users select the $X$ basis, then $\gamma_{a,b} = \alpha_{a,b}$. The two output states, denoted $|\xi^{(0)}_X\rangle_{a_1 b_1}$ and $|\xi^{(1)}_X\rangle_{a_1 b_1}$, can be derived from Eq. (S16) and depend on the cases $\alpha_a = \alpha_b$ and $\alpha_a \neq \alpha_b$:

$$\alpha_a = \alpha_b : |\xi^{(0)}_X\rangle_{a_1 b_1} = |\psi^+\rangle_{a_1 b_1}, \tag{S17}$$

$$\alpha_a \neq \alpha_b : |\xi^{(1)}_X\rangle_{a_1 b_1} = |\psi^-\rangle_{a_1 b_1}. \tag{S18}$$

If the users select the $Y$ basis, then $\gamma_{a,b} = \alpha_{a,b} + \pi/2$. The resulting output states $|\xi^{(0)}_Y\rangle_{a_1 b_1}$ and $|\xi^{(1)}_Y\rangle_{a_1 b_1}$ are equal to those in the $X$ basis, as it can be easily verified:

$$\alpha_a = \alpha_b : |\xi^{(0)}_Y\rangle_{a_1 b_1} = |\psi^+\rangle_{a_1 b_1}, \tag{S19}$$

$$\alpha_a \neq \alpha_b : |\xi^{(1)}_Y\rangle_{a_1 b_1} = |\psi^-\rangle_{a_1 b_1}. \tag{S20}$$

The above equations show the in-principle security of the scheme in Fig. S1e. The state emitted by the users, *before* any measurement is performed by Eve, is equal to either $|\psi^+\rangle_{a_1 b_1}$ or $|\psi^-\rangle_{a_1 b_1}$. The only information conveyed by these sates is the sign, which can only tell Eve whether the users encoded equal bits, associated with $|\psi^+\rangle_{a_1 b_1}$, or different bits, associated with $|\psi^-\rangle_{a_1 b_1}$. However Eve remains clueless about the absolute bit value encoded by each user, which depends on the single variables $\gamma_{a,b}$. These variables do not appear in Eqs. (S17)-(S20), only their difference does. So the output states do not depend on the individual phase values $\gamma_{a,b}$ but only on their difference $\gamma_b - \gamma_a$, as can also be seen from the output state in Eq. (S16). On the other hand, any attempt at measuring the state of a single user will leave Eve clueless about the correlations between the bits. This is seen, e.g., by tracing the state in Eq. (S16) over Alice's degrees of freedom, which returns a mixed state that does not contain phase information any more.

Each legitimate user, however, can easily retrieve the bit value of the other user from the result of Eve's measurement and the knowledge of their own bit value. In fact, the states $|\xi_X^{(0)}\rangle_{a_1b_1}$, $|\xi_Y^{(0)}\rangle_{a_1b_1}$ will trigger the detector D0, whereas the states $|\xi_X^{(1)}\rangle_{a_1b_1}$, $|\xi_Y^{(1)}\rangle_{a_1b_1}$ will trigger D1:

$$|\xi_X^{(0)}\rangle_{a_1b_1} = |\xi_Y^{(0)}\rangle_{a_1b_1} = |\mathrm{D0}\rangle_{a_1b_1}, \tag{S21}$$

$$|\xi_X^{(1)}\rangle_{a_1b_1} = |\xi_Y^{(1)}\rangle_{a_1b_1} = |\mathrm{D1}\rangle_{a_1b_1}. \tag{S22}$$

At this point, one remark is in order. In Fig. S1e we drew dashed-line boxes representing unitary operations to encode the random phase $\rho$. These are the same operations as in Figs. S1d ($\rho$ between points 1 and 2) and S1c ($\rho$ between points 2 and 3). If the users implemented such operations in the scheme of Fig. S1e, the security of the scheme would be unchanged. If the unitaries $\hat{U}_{a,b}^{(\rho)}$ were implemented between points 2 and 3 in Fig. S1e, this conclusion would be apparent from Eq. (S16). If $\hat{U}_{a,b}^{(\rho)}$ were implemented between points 1 and 2, the conclusion would easily follow from the relation

$$e^{i\rho}|n\rangle = |n\rangle. \tag{S23}$$

In other terms, the encoding of the random phase $\rho$ through the unitaries $\hat{U}_{a,b}^{(\rho)}$ is not at variance with the use of a perfect photon number source in the scheme of Fig. S1e. Even if the global phase $\rho$ is announced in this scheme, the users could have used, in principle, a photon number source to prepare the state seen by Eve. Hence, it is legitimate to consider this source to prove the security of the scheme of Fig. S1e.

## Actual schemes (Figs. S2a, S2b)

In the execution of the TF-QKD protocol, the bases are publicly announced and all the events with mismatched bases are discarded. Hence it suffices to consider only the events with matched bases and we analyse the two bases $X$ and $Y$ separately.

When the $X$ basis is selected, the transmitter in Fig. S1e is equivalent to the one in Fig. S2a. Here, each user owns an ancillary single-photon state, labelled $a_2$ for Alice and $b_2$ for Bob, which is not accessible to Eve. The users initially prepare the ancillary states in $|z_+\rangle$ to then measure them along the $X$ direction, through the measurement $\mathcal{M}_X$. Because the observables $Z$ and $X$ are complementary, they obtain a perfectly random outcome. If the outcome is $|x_+\rangle$ ('+' sign in Fig. S2a), they encode the phases $\gamma_{a,b} = 0$ (bit value 0, see step 3 of the TF-QKD protocol) on the paths $a_1$ and $b_1$. If the outcome is $|x_-\rangle$ ('−' sign in Fig. S2a), they encode the phases $\gamma_{a,b} = \pi$ (bit value 1) on $a_1$ and $b_1$. It is easy to verify that the quantum states at points 1, 2 and 3 of Fig. S2a are the same as the corresponding states in Fig. S1e when $\gamma_{a,b}$ runs on the $X$-basis values. In particular, when the outcome of $\mathcal{M}_X$ is '+' ('−'), the state at point 3 of Fig. S2a coincides with the state $|\xi_X^{(0)}\rangle$ ($|\xi_X^{(1)}\rangle$) given in Eq. (S17) (Eq. (S18)).

For the $Y$ basis, a similar argument applies. The corresponding scheme is now depicted in Fig. S2b. The users still prepare their ancillary states as $|z_+\rangle$, but they measure them along $Y$ ($\mathcal{M}_Y$ in the figure). If $|y_+\rangle$ is obtained ('+' sign in Fig. S2b), they encode the phase $\gamma_{a,b} = \pi/2$ (bit value 0 in the $Y$ basis) on the paths $a_1$ and $b_1$, whereas if $|y_-\rangle$ is obtained ('−' sign in Fig. S2b), they encode the phase $\gamma_{a,b} = 3\pi/2$ (bit value 1) on $a_1$ and $b_1$. It is easy to verify that the quantum states at points 1, 2 and 3 of Fig. S2b are the same as the corresponding points in Fig. S1e when $\gamma_{a,b}$ runs on the $Y$-basis values. In particular, when the outcome of $\mathcal{M}_Y$ is '+' ('−'), the output state (point 3 of Fig. S2b) coincides with the state $|\xi_Y^{(0)}\rangle$ ($|\xi_Y^{(1)}\rangle$) given in Eq. (S19) (Eq. (S20)).

This shows that the schemes in Figs. S2a and S2b are equivalent to the transmitter in Fig. S1e for matching bases. They implement the actual operations prescribed by TF-QKD and allow to measure the bit-error rates of the protocol. The $Y$-basis bit-error rate is obtained from the bits disclosed by the users during the public discussion whereas the $X$-basis bit-error rate becomes available during the error correction stage.

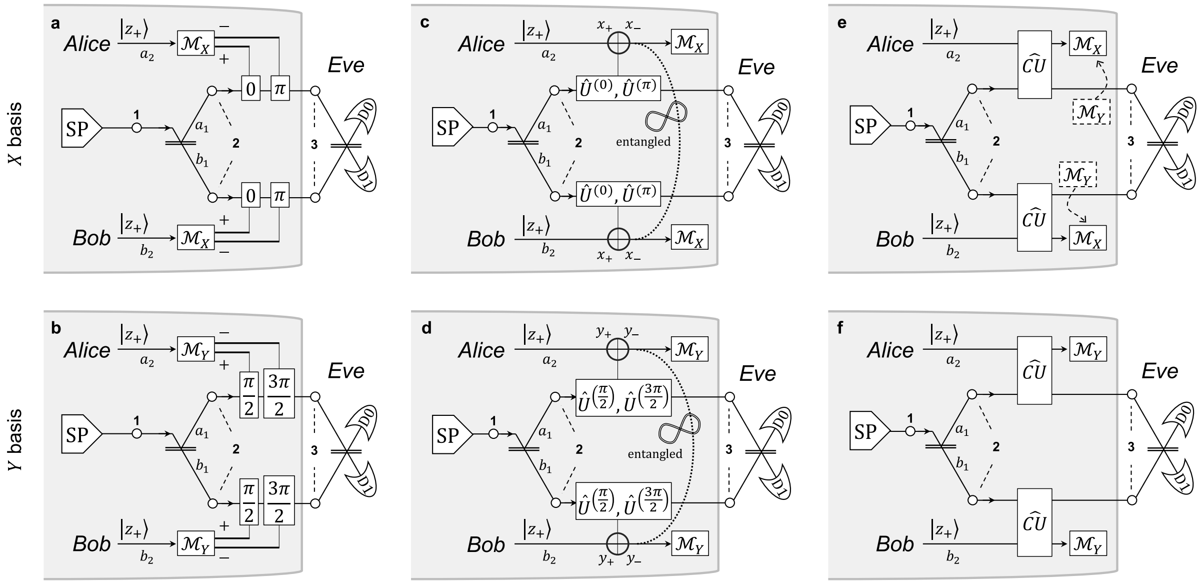


Figure S2: **Entanglement-based representation of TF-QKD.** The grey-shaded areas are inaccessible to Eve. **a**, **b**, Single-photon representation of the actual protocol in the $X$ and $Y$ basis, respectively. The key bits are distilled from the $X$ basis whereas the $Y$ basis is used to test the channel. **c**, **d**, Schemes resulting from postponing the measurements $\mathcal{M}_X$ and $\mathcal{M}_Y$, respectively, until after the announcement of Eve's measurement's results. Entanglement is distributed between Alice and Bob via a single photon that is initially split and then recombined at the central measuring station. **e**, **f**, Virtual schemes to identify and estimate the phase-error rate in the $X$ basis. For $X$ and $Y$ complementary bases, a phase error can be found by measuring the $X$-basis states in the $Y$ basis (Fig. S2e). The phase-error rate coincides with the bit-error rate of a $Y$-basis state measured in the $Y$-basis (Fig. S2f) if the only difference between the schemes in Figs. S2e and S2f is the measuring basis of the ancillary states on paths $a_2$ and $b_2$.

## Entanglement distillation and virtual schemes (Figs. S2c – S2f)

We now observe that all the outcomes in the protocol would not change if Alice and Bob delayed their measurements $\mathcal{M}_X$ and $\mathcal{M}_Y$ until after the announcement of Eve's measurement's results. The corresponding schemes are depicted in Figs. S2c for the $X$ basis and S2d for the $Y$ basis.

Let us consider the $X$ basis first. In the configuration of Fig. S2c, we have the following controlled operations:

$$\hat{\mathrm{C}U}^{(X)}_{a_{12}} = \hat{U}^{(0)}_{a_1} \otimes |x_+\rangle_{a_2}\langle x_+| + \hat{U}^{(\pi)}_{a_1} \otimes |x_-\rangle_{a_2}\langle x_-|, \tag{S24}$$

$$\hat{\mathrm{C}U}^{(X)}_{b_{12}} = \hat{U}^{(0)}_{b_1} \otimes |x_+\rangle_{b_2}\langle x_+| + \hat{U}^{(\pi)}_{b_1} \otimes |x_-\rangle_{b_2}\langle x_-|. \tag{S25}$$

With these operators, the phase encodings on paths $a_1$ and $b_1$ are executed conditional on the state of the control qubits on $a_2$ and $b_2$. These are the ancillary states owned by the users, which are prepared in the superposition of $X$-basis states $|z_+\rangle = (|x_+\rangle + |x_-\rangle)/\sqrt{2}$. By applying the operations in Eqs. (S24), (S25) to the initial state $|\psi^+\rangle_{a_1b_1}$ we obtain:

$$\begin{aligned} |\lambda_X\rangle_{ab} &= \left[\hat{\mathrm{C}U}^{(X)}_{b_{12}}\right]\left[\hat{\mathrm{C}U}^{(X)}_{a_{12}}\right]|\psi^+\rangle_{a_1b_1}|z_+\rangle_{a_2}|z_+\rangle_{b_2} \\ &= \left[\hat{U}^{(0)}_{b_1}|x_+\rangle_{b_2} + \hat{U}^{(\pi)}_{b_1}|x_-\rangle_{b_2}\right]\left[\hat{U}^{(0)}_{a_1}|x_+\rangle_{a_2} + \hat{U}^{(\pi)}_{a_1}|x_-\rangle_{a_2}\right]\left(|1\rangle_{a_1}|0\rangle_{b_1} + |0\rangle_{a_1}|1\rangle_{b_1}\right)/(2\sqrt{2}) \\ &= \left(|\mathrm{D}0\rangle_{a_1b_1}|\Phi^-_X\rangle_{a_2b_2} + |\mathrm{D}1\rangle_{a_1b_1}|\Psi^-_X\rangle_{a_2b_2}\right)/\sqrt{2}. \end{aligned} \tag{S26}$$

If the users measure the state in Eq. (S26) in the $X$ basis on paths $a_2$ and $b_2$, they will project it into the same states $|\xi_X^{(0)}\rangle$, $|\xi_X^{(1)}\rangle$ of the previous scheme, Fig. S1a, see Eqs. (S21), (S22). This shows the equivalence of the two preparations. The states $|\Psi_X^-\rangle_{a_2 b_2}$, $|\Phi_X^-\rangle_{a_2 b_2}$ are two of the four Bell states defined in Eqs. (S6) and (S7), which are maximally entangled. This shows that Eve's measurement leaves the ancillary states on $a_2$ and $b_2$ in a maximally entangled state, which coincides with the Bell state $|\Phi_X^-\rangle$ or $|\Psi_X^-\rangle$ depending on which detector clicks. Because these states are pure, they are necessarily disentangled from any other state. Moreover, they are maximally entangled, so the users could in principle measure their halves of the entangled state (Alice on $a_2$, Bob on $b_2$) and retrieve the bit information in a secure way. This is the same argument used in the security proof of the standard BB84 protocol.[47,56]

More specifically, to enable the distillation protocol, the users have to detect and correct bit and phase errors in a set of noisy entangled pairs. This is possible in principle in the BB84 protocol because the corresponding measurements commute.[56] Then, by using specific quantum error correction codes,[58,59] the users can bypass the correction of the phase errors, provided that they manage to show that the phase-error rate in their scheme is small enough.[47] Therefore proving the security of BB84 is reduced to reliably estimate the phase-error rate of the protocol.

We follow here the same approach. The users could agree that every time Eve announces the state $|\mathrm{D1}\rangle$, Bob flips his state before measuring it. This turns a $|\Psi_X^-\rangle$ state into a $|\Phi_X^-\rangle$ state, which could then represent the target state for the entanglement distillation protocol.[60] If during the execution of this protocol the users find an error rate above the tolerable threshold, they will abort. Otherwise, they will manage to in principle distill maximally entangled states out of a set of corrupted initial states. When maximally entangled states become available, the users can measure them and get the key bits with absolute security.

Let us notice that, in this perspective, it does not matter *how* the ancillary states shared by Alice and Bob were initially corrupted, whether the natural noise of the channel introduced some decoherence or whether Eve tried to attack the channel. Irrespective of the real cause, when the distillation protocol is successful, the final state is guaranteed to be secure. By a similar argument, it does not matter whether Eve actually performed the measurement prescribed by the TF-QKD protocol, or whether she disclosed the true results. When Eve publicly announces the results, she commits herself to well-defined classical variables. The users can then test their bit-error and phase-error rate estimates against the outcomes announced by Eve and abort the protocol if they are too large. If they do not abort, they will distill a secure key with high probability.

The element that remains to be proven is that the users can estimate the phase-error rate in the computational basis $X$ by measuring the bit-error rate in the $Y$ basis. For that, let us first notice that we can repeat for the $Y$ basis the same argument presented for the $X$ basis. The controlled operations in the diagram of Fig. S2d, which depend on the ancillary state $|y_+\rangle$ or $|y_-\rangle$, are represented by the following operators:

$$\begin{aligned}
\mathrm{C}\hat{U}_{a_{12}}^{(Y)} &= \hat{U}_{a_1}^{(\frac{\pi}{2})} \otimes |y_+\rangle_{a_2}\langle y_+| + \hat{U}_{a_1}^{(\frac{3\pi}{2})} \otimes |y_-\rangle_{a_2}\langle y_-|, \\
\mathrm{C}\hat{U}_{b_{12}}^{(Y)} &= \hat{U}_{b_1}^{(\frac{\pi}{2})} \otimes |y_+\rangle_{b_2}\langle y_+| + \hat{U}_{b_1}^{(\frac{3\pi}{2})} \otimes |y_-\rangle_{b_2}\langle y_-|.
\end{aligned}$$

By applying them to the initial state we obtain:

$$\begin{aligned}
|\lambda_Y\rangle_{ab} &= \left[\mathrm{C}\hat{U}_{b_{12}}^{(Y)}\right]\left[\mathrm{C}\hat{U}_{a_{12}}^{(Y)}\right]|\psi^+\rangle_{a_1 b_1}|z_+\rangle_{a_2}|z_+\rangle_{b_2} \\
&= -\frac{i}{\sqrt{2}}\left(|\mathrm{D0}\rangle_{a_1 b_1}|\Phi_Y^-\rangle_{a_2 b_2} + |\mathrm{D1}\rangle_{a_1 b_1}|\Psi_Y^-\rangle_{a_2 b_2}\right).
\end{aligned}$$

From Eqs. (S10), (S11) it follows that $|\lambda_X\rangle$ and $|\lambda_Y\rangle$ are indistinguishable:

$$\langle\lambda_X|\lambda_Y\rangle = 1. \tag{S27}$$

The same result could have been obtained from the definition of the complementary bases $X$ and $Y$, i.e., by rewriting the eigenstates of $X$ as $|x_\pm\rangle = \left(e^{\mp i\frac{\pi}{4}}|y_+\rangle + e^{\pm i\frac{\pi}{4}}|y_-\rangle\right)/\sqrt{2}$ and replacing them in Eq. (S26).

Hence the two basis-dependent operators $\hat{CU}^{(X)}$ and $\hat{CU}^{(Y)}$ are the same operator, which we denote with the basis-independent label $\hat{CU}$ in Figs. S2e and S2f. Then if the ancillary states on $a_2$ and $b_2$ were measured in the $Y$ basis rather than in the $X$ basis the final result would not change. The users could even decide the measurement basis *after* Eve has announced her results, without affecting the outcomes. Therefore, Eve's information does not change if the users decided to replace the measurement $\mathcal{M}_X$ with $\mathcal{M}_Y$, leaving everything else unchanged. This guarantees that the scheme in Fig. S2e is equivalent to the scheme in Fig. S2f. In turn, because the scheme in Fig. S2f is equivalent to the actual scheme in Fig. S2b, we conclude that the $X$-basis phase-error rate can be reliably estimated from the bit-error rate measured in the $Y$ basis.

We can now borrow the remaining part of the security proof from the one developed for the BB84 protocol and guarantee the security of the scheme in Fig. S1e. For sufficiently low error rates, the users could in principle distill states that are pure and maximally entangled, therefore necessarily uncorrelated from any other party. This virtual protocol can be eventually reduced to one where only the actual operations are performed. In our description, this corresponds to the schemes in Figs. S2a ($X$ basis) and S2b ($Y$ basis), which have been shown to be equivalent to the one in Fig. S1e. Moreover, standard error correction[61,62] and privacy amplification[63,64] replace the quantum error correction of bit-flip and phase-flip errors. This leads to the following rate equation for the scheme in Fig. S1e:

$$R_{(\text{Fig. S1e})} = \omega_{\text{sift}} \left[1 - h(e_1^{\text{bit}}) - h(e_1^{\text{ph}})\right], \tag{S28}$$

with $e_1^{\text{bit}}$ and $e_1^{\text{ph}}$ the single-photon bit and phase error rates of the protocol, respectively, and $\omega_{\text{sift}}$ a coefficient due to the sifting of $\rho_{ba}$. In the above equation, it has been assumed that the fraction of bits devoted to testing the channel against Eve's presence is asymptotically negligible. It is worth noting that if the users encoded the phase $\rho$ as shown in Fig. S1e (dashed boxes), the argument developed in this section and in the previous one would still apply, by virtue of the discussion related to Eq. (S23).

## Weak-coherent-pulse source

In the previous section we derived the secure key rate of the single-photon scheme in Fig. S1e. However, the security of TF-QKD depends on the scheme in Fig. S1d, which features a different light source. Here the single-photon source is replaced by a laser emitting weak coherent pulses followed by a block that randomises the electromagnetic phase of the emitted states.

When we go from Fig. S1e back to Fig. S1d, we must include in the security analysis the announcement of the global random phase $\rho$. In the virtual scheme of Fig. S1d, the announcement of $\rho$ is not required to reconcile the phases and the users only need to know $\rho_{ba}$ to sift their data. However, in the actual protocol, the users need to exchange both $\rho_a$ and $\rho_b$ to determine the value of $\rho_{ba}$ and this corresponds, in the scheme of Fig. S1d, to disclosing $\rho$. The security of TF-QKD after disclosing $\rho$ is a subtle issue and we devote the next sections to discuss this point in detail.

We start by analysing the security of the protocol under the following assumption:

$A^{(\neg\rho)}$: THE GLOBAL PHASE $\rho$ DOES NOT LEAK INFORMATION TO THE EAVESDROPPER.

The negation of $\rho$ in the superscript reminds that the global phase $\rho$ plays no role in security until the above assumption is enforced. Then, in the next section, we drop this assumption and examine how this can affect the security of the scheme.

When the assumption $A^{(\neg\rho)}$ is enforced, Eve gains no information from $\rho$, as she is in the same position as when $\rho$ remains fully undisclosed, like in the BB84 protocol. So we can use the *tagging*[25] argument to connect the perfect source in Fig. S1e with the practical one in Fig. S1d.

According to the description of TF-QKD in the virtual protocol, in every run the value of $\rho$ is picked at random in the interval $[0, 2\pi)$. Therefore the density matrix $\hat{\sigma}$ prepared by the users in the scheme of

Fig. S1d, as it would be seen by Eve, is:[25,65,70–72]

$$\hat{\sigma} = \frac{1}{2\pi}\int_0^{2\pi} d\rho |e^{i\rho}\sqrt{\mu}\rangle\langle e^{i\rho}\sqrt{\mu}| \quad \text{(S29)}$$

$$= \sum_{n=0}^{\infty} p_{n|\mu}|n\rangle\langle n| \quad \text{(S30)}$$

$$= f_{\rm unt}\hat{\sigma}_{\rm unt} \oplus f_{\rm tag}\hat{\sigma}_{\rm tag}, \quad \text{(S31)}$$

where $p_{n|\mu} = e^{-\mu}\mu^n/n!$ and we have set

$$f_{\rm unt}\hat{\sigma}_{\rm unt} = e^{-\mu}|0\rangle\langle 0| + \mu e^{-\mu}|1\rangle\langle 1|, \quad \text{(S32)}$$

$$f_{\rm tag}\hat{\sigma}_{\rm tag} = e^{-\mu}\sum_{n=2}^{\infty}\frac{\mu^n}{n!}|n\rangle\langle n|, \quad \text{(S33)}$$

with $f_{\rm tag} = 1 - f_{\rm unt} = 1 - e^{-\mu} - \mu e^{-\mu}$ representing the probability that a pulse jointly prepared by the users contains more than one photon. Multi-photon pulses leak basis information to the eavesdropper, so they are "tagged",[25] or "taggable", by Eve. The worst possible case is when tagged pulses leak full information to Eve and this is the case normally considered in security proofs. On the other hand, zero-photon and single-photon states, defining $\hat{\sigma}_{\rm unt}$, are basis-independent and leak no information to Eve. Therefore, it follows that all the security results proven for the single-photon scheme in Fig. S1e also hold for the TF-QKD scheme under the condition that $A^{(\neg\rho)}$ holds, limited to the fraction of untagged bits.[25,50]

More specifically, Eq. (S31) justifies an interpretation where the users classify each preparation as either taggable or untaggable. This lets them bound the untagged fraction $\Omega_{\rm unt}$ of detection events that have originated from zero-photon or single-photon signals. The resulting key rate can then be written as[22,25]

$$R_{\rm unt} = \omega_{\rm sift}Q_\mu\left\{\Omega_{\rm unt}\left[1 - h\left(\frac{E_\mu}{\Omega_{\rm unt}}\right)\right] - h(E_\mu)\right\}, \quad \text{(S34)}$$

where $Q_\mu$ and $E_\mu$ are the measured gain and QBER of the pulses with intensity $\mu$ and we have maintained the sifting factor $\omega_{\rm sift}$ due to the presence of $\rho_{ba}$.

If we limit the untagged bits to the single-photon pulses, neglecting the (usually small) contribution of the zero-photon pulses, then $\Omega_{\rm unt} = Q_1/Q_\mu$ and the above key rate can be rewritten as

$$R_{\rm unt} = \omega_{\rm sift}\left\{Q_1\left[1 - h\left(\frac{Q_\mu E_\mu}{Q_1}\right)\right] - Q_\mu h(E_\mu)\right\}, \quad \text{(S35)}$$

where $Q_1$ represents the gain of the single-photon, hence untaggable, pulses emitted by the users.

The decoy state technique[20] makes it possible to bound the single-photon quantities in Eqs. (S34) and (S35) with high accuracy.[21,22] We denote $\underline{\Omega}_{\rm unt}$ and $\underline{Q}_1$ the lower bounds for the fraction of untagged bits and for the single-photon gain, respectively, and $\overline{e}_1$ the upper bound for the single-photon QBER. Eq. (S34) then becomes[21]

$$R_{\rm unt} \geq \omega_{\rm sift}Q_\mu\left\{\underline{\Omega}_{\rm unt}\left[1 - h\left(\frac{E_\mu}{\underline{\Omega}_{\rm unt}}\right)\right] - h(E_\mu)\right\}, \quad \text{(S36)}$$

and Eq. (S35) becomes[22]

$$R_{\rm unt} \geq \omega_{\rm sift}\left\{\underline{Q}_1\left[1 - h\left(\overline{e}_1\right)\right] - Q_\mu h(E_\mu)\right\}. \quad \text{(S37)}$$

The above equations represent two different bounds to the actual key rate: Eq. (S37) is tighter, but requires the estimation of the single-photon QBER, which is not required in Eq. (S36). In the following, we only discuss Eq. (S37), but all the arguments apply unchanged to Eq. (S36) as well.

Our next claim is that, under the assumption $A^{(\neg\rho)}$:

1. When the IM is not employed, the scheme in Fig. S1d can achieve the key rate in Eq. (S34), where the untagged fraction is bounded by $\Omega_{\mathrm{unt}} \geq 1 - f_{\mathrm{tag}}/Q_\mu$.
2. When the IM is employed, the scheme in Fig. S1d can achieve the better key rate in Eq. (S37), with the single-photon quantities estimated through the decoy state technique.

To support our claim, we notice that the scheme in Fig. S1d is the same transmitter as in the BB84 protocol, for which the key rates have been given in [25,50], when the IM is not included, and in [22], when the IM is included. In particular, for the decoy-state key rate related to the scheme in Fig. S1d, we notice that one of the fundamental assumptions of this technique, the randomisation of the initial state's electromagnetic phase, is guaranteed by the presence of the phase randomiser, whereas the possibility to modulate the intensity is guaranteed by the presence of the IM. Moreover, by virtue of Eq. (S30), the fundamental decoy-state equations[22] hold for this scheme, because the signal or decoy classes are indistinguishable to Eve.

Therefore, under $A^{(\neg\rho)}$, we can apply the usual decoy-state equations to the transmitter in Fig. S1d and obtain the key rate in Eqs. (S36) or (S37). We incidentally notice that the application of decoy states to a setup where Eve performs the measurements and the users exploit her results to distil key bits is not new and represents a basic tool in MDI-QKD.[23] We also notice that in the BB84 protocol the squashing model[25,73,74] is adopted to guarantee that Bob's measurement's limited efficiency does not introduce a dependance on the basis in the state sent by Alice, thus enhancing Eve's information.[71] However, in TF-QKD and in the scheme of Fig. S1d, this is not needed as Bob is a transmitter and the detectors are controlled by Eve.

The key rate for TF-QKD under assumption $A^{(\neg\rho)}$ is now obtained by noting that, due to the reduction argument previously described, its security is at least as strong as the scheme in Fig. S1d. The key rate is therefore given by Eq. (S37), to which we have to add the peculiar sifting mechanisms of TF-QKD. There is an overall sifting factor due to the reconciliation of the random phases (factor $1/M$) and one due to the fulfillment of the locking condition (factor $d$). We then add a coefficient $f \geq 1$ to take the inefficiency of the error correction into account.[22] Finally, we express the key rate assuming that the users perform a refined data analysis,[26] counting the detection events and the errors separately in the two bases. This is legitimate[75] as, limitedly to the untagged states, the protocol is basis-independent, so splitting the detected sample according to the basis represents a fair sampling of the overall data set. When we gather these elements into a single equation we get

$$R^{(\neg\rho)}_{\text{TF-QKD}} = \frac{d}{M}\left\{\underline{Q}_1\left[1 - h\left(\overline{e}_1\right)\right] - fQ_\mu h(E_\mu)\right\}, \tag{S38}$$

which is Eq. (3) in the main text. This rate equation is formally equal to the one used for the efficient decoy-state BB84 protocol. We can therefore generally use it in the same way. However, it is worth remarking that, similarly to the BB84 protocol, the distance between the preparation stage and the detection stage is $L$, but, differently from the BB84 protocol, the distance between Alice and Bob is $2L$.

Before we conclude this section, it is convenient for later use to rewrite Eq. (S38) in terms of the information gained by each party, as follows:

$$\begin{aligned} R^{(\neg\rho)}_{\text{TF-QKD}} &= \frac{d}{M}Q_\mu\left\{1 - fh(E_\mu) - \left[1 - \frac{\underline{Q}_1}{Q_\mu}\left(1 - h\left(\overline{e}_1\right)\right)\right]\right\} \\ &= \frac{d}{M}Q_\mu\left[I_{AB} - \overline{I}_E^{(\neg\rho)}\right], \end{aligned} \tag{S39}$$

where $I_{AB} = 1 - fh(E_\mu)$ is the mutual information between Alice and Bob and $\overline{I}_E^{(\neg\rho)} = 1 - \underline{Q}_1/Q_\mu(1 - h\left(\overline{e}_1\right))$ is the upper bound for Eve's information under the assumption $A^{(\neg\rho)}$.

# Dropping the assumption on random phase announcement

In the previous section, we analysed the security of TF-QKD under the assumption that the announcement of the global phase $\rho$ does not leak information to the eavesdropper. In this section, we describe how

removing this assumption can affect the protocol's security.

However, before dropping $A^{(\neg\rho)}$, let us show some examples where $A^{(\neg\rho)}$ holds, or partially holds.

A first example is when Eve is limited to perform a measurement based on photodetection. If Eve applies photodetection to the pulses emitted by the users, she projects the resulting states into a density matrix that is diagonal in the photon number states. Therefore, the information carried by $\rho$ is erased and Eve cannot exploit it anymore. This situation includes, for instance, the photon-number-splitting (PNS) attack,[65] which is the most powerful attack against the phase-randomised BB84 protocol, and the conditional beam splitting attack,[66] which approximates the PNS with a series of beam splitters followed by conditional photodetection.

A second example where the assumption $A^{(\neg\rho)}$ clearly holds is when $\rho$ remains undisclosed. For example, the users could encrypt the global phase information with the one-time pad[67] thus making it unavailable to Eve. Of course, because the global phase information is much larger than the key distilled in the protocol, there is no key gain in this version of the protocol. However, the global phase is encoded on quantum states and we cannot exclude the possibility that the users can recycle the one-time-pad key,[68] thus achieving a net gain. An interesting variant of this method is if the users adapt TF-QKD to accept a discrete global phase randomisation.[69] In this case, they could decide in advance the values of the global phase and recycle this sequence of values until it becomes too degraded to be reused. This latter method would also enhance the sifting efficiency, hence the key rate, of TF-QKD.

Let us now study how dropping the assumption $A^{(\neg\rho)}$ can affect the security of the TF-QKD scheme presented in the main text. To tackle this problem, it is convenient to maintain the virtual description where the global phase is split into $\rho$ and $\rho_{ba}$. We can then give $\rho_{ba}$ to Eve and reduce the security issue to publicly revealing $\rho$. The users do not really need to reveal $\rho$ in the virtual protocol, as the sifting of their data depends on $\rho_{ba}$. However, the disclosure of $\rho$ is necessary to make the virtual protocol equivalent to the actual one, where $\rho_a$ and $\rho_b$ are fully revealed.

When the global phase $\rho$ is revealed, Eve's knowledge about the source of quantum states generally increases. In particular, after the announcement of the global phase, it is not possible any more to write the density matrix of the users' states as a photon number channel, as in Eq. (S31). This suggest that the key rate $R^{(\neg\rho)}_{\text{TF-QKD}}$ is an over-optimistic prediction of the true TF-QKD key rate.

On the other hand, it is crucial to observe the temporal sequence of the events. The global phase is only disclosed after the quantum communication is over, after Eve has announced the results of her measurement and after the bases have been disclosed by the users. This entails some relevant consequences.

The first is that Eve cannot exploit the global phase information to enhance her real-time attack of the signals traveling along the channel. At the time of the measurement, Eve ignores $\rho$ and faces the same situation as in the presence of the assumption $A^{(\neg\rho)}$. The second is that Eve's announcement cannot depend on the global phase. Therefore, transmission and error rates measured by the users cannot depend on $\rho$ either. Finally, the announcement of $\rho$ cannot give Eve more basis information than she already has. Because $\rho$ is disclosed after the bases are revealed, Eve already knows all the bases used in the protocol.

However, we cannot exclude the possibility that the announcement of $\rho$ leaks bit information to Eve. Clearly, the bit information is always useful to the eavesdropper, even after all the measurements have been completed, because it directly relates to the secret key. For example, if the users announced directly the bits, the security of the protocol would be clearly compromised. A less trivial situation is when the announcement of the global phase allows Eve to post-select a restricted number of ancillary states that she can correlate with the key bits. This possibility is described with an explicit example in the next section.

## Collective beam-splitting attack

Here, we analyse the situation where the announcement of the global phase allows Eve to extract additional information from her ancillary states.

A powerful example of this possibility is given by the collective beam-splitting (CBS) attack. This was described in relation to a binary continuous-variable protocol[76] and to phase-distributed protocols.[77]

Here, we adapt it to TF-QKD.

In the CBS attack, Eve uses two identical beam splitters, placed on the paths connecting Alice and Bob to the measuring station, to extract part of the signals from the communication channel. The beam splitters have transmission $t = \sqrt{\eta}$ and reflection $r = \sqrt{1-\eta}$, where $\eta$ is the transmission of the channels connecting the users to the measuring station. Eve stores all the states reflected by the beam splitters on her ancillae and uses the states transmitted by the beam splitters to announce her measurement's results during the step 4 of the TF-QKD protocol. Because the transmission of the beam splitters coincides with the channel transmission, the users will not notice any unusual loss in their system. Also, because the signals transmitted through the beam splitters are not perturbed by Eve, the users will not notice an increase in the QBER. This illustrates the dangerousness of this attack.

After the quantum transmission, Eve's ancillae will be correlated with the states emitted by the users, given in Eq. (S15). Their state will be:

$$|e^{i\gamma_a} e^{i\rho} \sqrt{(1-\eta)\mu_a}\rangle_{e_a} |e^{i\gamma_b} e^{i\rho} \sqrt{(1-\eta)\mu_b}\rangle_{e_b}, \tag{S40}$$

where we denoted $e_a$ and $e_b$ Eve's ancillae on Alice's and Bob's paths, respectively.

At the step 5 of the protocol, the global phase $\rho$ and the bases, contained in the variables $\gamma_{a,b}$, are announced, whereas the bit values are kept secret. After all the mismatched events are discarded, both by the users and by Eve, the remaining states in the eavesdropper's hands will be

$$| \pm \sqrt{(1-\eta)\mu_a}\rangle_{e_a} | \pm \sqrt{(1-\eta)\mu_b}\rangle_{e_b}, \tag{S41}$$

where we associate the $+$ $(-)$ sign with the bit value 0 (1).

From the measurement of the states transmitted through the beam splitters, Eve also knows whether the users encoded equal or different bit values. This information is in fact disclosed by Eve herself during the step 4 of the TF-QKD protocol. Suppose that the encoded bits are equal (the case with different bits is analogous). In this case the signs in the states of Eq. (S41) are equal, so Eve can learn the bit value by discriminating between the following two states:

$$|\psi_0\rangle_e = |\sqrt{(1-\eta)\mu_a}\rangle_{e_a} |\sqrt{(1-\eta)\mu_b}\rangle_{e_b}, \tag{S42}$$

$$|\psi_1\rangle_e = |-\sqrt{(1-\eta)\mu_a}\rangle_{e_a} |-\sqrt{(1-\eta)\mu_b}\rangle_{e_b}, \tag{S43}$$

where the subscripts 0 and 1 refer to the bit values.

Several bounds are available to estimate Eve's success probability in discriminating between the above states,[78] for instance, the minimum-error-discrimination bound[79] and the unambiguous-state-discrimination bound.[80–82] These bounds, however, are all related to a discrimination between individual ancillary states. Here, on the contrary, we want to give Eve more resources and estimate the maximum information she can get by performing a collective measurement on her ancillae. In this case, the maximum information she can extract is upper bounded by the Holevo quantity:[83,84]

$$I_E^{(\mathrm{CBS})} \le \overline{I}_E^{(\mathrm{CBS})} = S(\hat{r}) - \frac{1}{2}[S(\hat{r}_0) + S(\hat{r}_1)], \tag{S44}$$

where $\overline{I}_E^{(\mathrm{CBS})}$ is the upper bound to Eve's information in the CBS attack; $\hat{r}_0 = |\psi_0\rangle_e\langle\psi_0|$, $\hat{r}_1 = |\psi_1\rangle_e\langle\psi_1|$, $\hat{r} = (\hat{r}_0 + \hat{r}_1)/2$ and $S(\hat{x}) = -\mathrm{tr}(\hat{x}\log_2 \hat{x})$ represents the von Neumann entropy of the quantum state $\hat{x}$.

The corresponding information can be explicitly calculated. The entropy of the pure states $\hat{r}_{0,1}$ is zero. The entropy of the state $\hat{r}$ is related to the scalar product of the states in Eqs. (S42), (S43) and is equal to

$$S(\hat{r}) = h\left[\frac{1-e^{-2(1-\eta)\mu}}{2}\right] = \overline{I}_E^{(\mathrm{CBS})}, \tag{S45}$$

where $\mu = \mu_a + \mu_b$. By virtue of Eq. (S44), the above quantity represents the maximum information Eve can get from a CBS attack per detection event. If we add this information to the one Eve gets before

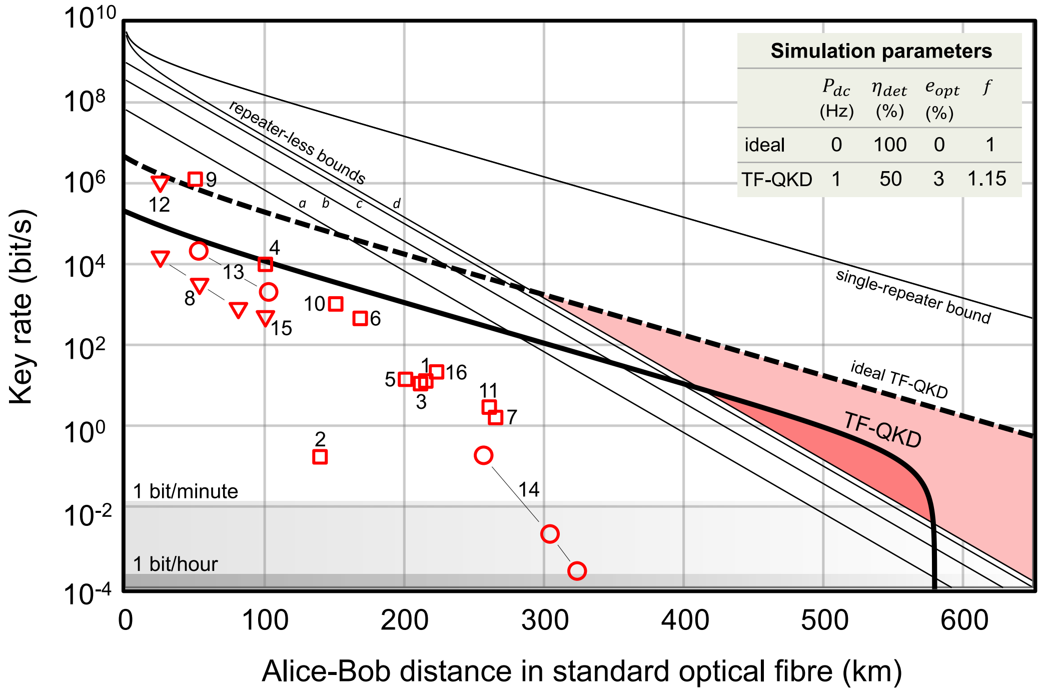


Figure S3: **TF-QKD key rates with the addition of collective beam splitting (CBS) attack**. The curves have the same meaning as in Fig. 1a of the main text. The solid (dashed) line is for the realistic (ideal) TF-QKD key rate under the most general attack performed by Eve before the global phase announcement plus the CBS attack performed after the announcement. The key rates are slightly bent upwards at short distance because the CBS attack becomes more effective after 3 dB of the communication distance, where more pulses are directed towards Eve's ancillae than towards the central measuring station. After this initial tradeoff, the key rate is dominated by the CBS attack, which pushes the initial intensity set by the users towards low values. The close-to-optimal total intensity of the signals used in the simulation is 0.1 (0.05) for the ideal (realistic) TF-QKD implementation. Letter-code for the theoretical bounds are: *a*, decoy-state MDI-QKD; *b*, decoy-state QKD; *c*, single-photon QKD; *d*, secret key capacity. See section "Numerical simulations" for the explicit expressions. Symbol-code for the experimental results: squares, triangles and circles are for QKD, continuous-variable QKD and MDI-QKD, respectively. Inset: $P_{dc}$, dark count probability; $\eta_{det}$, total detection efficiency; $e_{opt}$, channel optical error rate; $f$, error correction coefficient. The simulation parameters related to detectors are different from Fig. 1a. Here, we considered $P_{dc} = 1$ Hz (10 Hz in Fig. 1a) and $\eta_{det} = 50\%$ (30% in Fig. 1a), which are still featured by commercially available single-photon detectors.[85,86]

the global phase is announced, $\overline{I}_E^{(\neg\rho)}$ in Eq. (S39), and draw the resulting key rate, we obtain the plots in Fig. S3, which is a new version of Fig. 1a in the main text.

It is apparent that, despite the additional substantial information gained by Eve through the CBS attack, the TF-QKD key rates still scale with the square-root of the channel's transmission. Hence, it is still possible to overcome the SKC bound at large distance, above 300 km (400 km) for the ideal (realistic) TF-QKD implementation. It is also worth noting that the new rates have been obtained without changing the simulation parameter corresponding to the protocol's optical noise, $e_{opt}$, showing that the demands on the optical alignment of the system are unchanged, even in the presence of the CBS attack. Other parameters have been modified to enhance the detection rate at long distance, as reported in the inset of Fig. S3. However, also the more technologically demanding simulation parameters correspond to commercially available single-photon detectors.[85,86]

## Considerations on the key rates in Fig. S3

Although the key rates in Fig. S3 have not been proven to be lower bounds for the TF-QKD key rates, common sense suggests that they are over-conservative in fact.

Before the global phase is announced, Eve's knowledge about the initial Alice-Bob state is described by the density matrix $\hat{\sigma}_{ab}^{(\mathrm{pre})} = \hat{\sigma}$, given in Eqs. (S29)–(S31). After the global phase is announced, Eve's knowledge is updated to the following density matrix:

$$\hat{\sigma}_{ab}^{(\mathrm{post})} = \frac{M}{2\pi} \int_0^{\frac{2\pi}{M}} d\rho \; \hat{P}(e^{i\rho}\sqrt{\mu}), \tag{S46}$$

where we have used the notation $\hat{P}(x) = |x\rangle\langle x|$ and we have considered that only the phase slices $\Delta_k$ are announced, not the exact global phase $\rho$, so Eve still has an uncertainty $2\pi/M$ on the phase value. This brings the width of a phase slice, $2\pi/M$, to the integral's upper limit.

Let us now suppose that Eve's strategy depends on the global phase announcement. She could prepare her ancillae in such a way that, before $\rho$ is announced, she gets maximum information $\overline{I}_E^{(\neg\rho)}$, as in Eq. (S39). Then, after $\rho$ is announced, she gets additional information $\Delta I_E^{(\rho)}$. This is what we considered to draw the TF-QKD key rates in Fig. S3, where we set $\Delta I_E^{(\rho)} = \overline{I}_E^{(\mathrm{CBS})}$. However, this already appears to be over-pessimistic, giving Eve more information than she can really get. The reason is that Eve's ancillae cannot simultaneously provide $\overline{I}_E^{(\neg\rho)}$ and $\overline{I}_E^{(\mathrm{CBS})}$.

To make this statement more precise, we connect $\Delta I_E^{(\rho)}$ to an optimal measurement and then show that the gained information is always smaller than the maximum information $\overline{I}_E^{(\mathrm{CBS})}$ extracted from the CBS attack (Eq. (S45)).

Our argument is that, regardless of how Eve prepares her ancillae, she will have to measure them in order to gain the information $\Delta I_E^{(\rho)}$. However, her most powerful measurement cannot give her more information than she would retrieve from the optimal measurement to distinguish $\hat{\sigma}_{ab}^{(\mathrm{pre})}$ from $\hat{\sigma}_{ab}^{(\mathrm{post})}$. In turn, the maximum probability to distinguish between two quantum states $\hat{x}$ and $\hat{y}$ with an optimal measurement is given by the trace distance $D(\hat{x}, \hat{y})$.[51,87] Therefore we can quantify the information gain as

$$\Delta I_E^{(\rho)} \leq 1 - h(p_{\mathrm{succ}}), \tag{S47}$$

where $p_{\mathrm{succ}} = 1/2[1 + D(\hat{x}, \hat{y})]$.[88] Because the trace distance is convex in each of its inputs, we can bound the trace distance between the states $\hat{\sigma}_{ab}^{(\mathrm{pre})}$ and $\hat{\sigma}_{ab}^{(\mathrm{post})}$ as follows:

$$\begin{aligned} D\left(\hat{\sigma}_{ab}^{(\mathrm{pre})}, \hat{\sigma}_{ab}^{(\mathrm{post})}\right) &\leq \frac{M}{4\pi^2} \iint_V d\rho\, d\rho' D\left[\hat{P}(e^{i\rho}\sqrt{\mu}), \hat{P}(e^{i\rho'}\sqrt{\mu})\right] \\ &= \frac{M}{4\pi^2} \iint_V d\rho\, d\rho' \sqrt{1 - e^{-2\mu[1-\cos(\rho'-\rho)]}}, \end{aligned} \tag{S48}$$

where $V$ specifies the domains $\rho \in [0, 2\pi]$ and $\rho' \in [0, 2\pi/M]$. By solving the above integral and plugging the result into Eq. (S47), we have verified that $\Delta I_E^{(\rho)}$ is always considerably smaller than $\overline{I}_E^{(\text{CBS})}$, for any value of the free parameter $\mu$, thus justifying our statement at the beginning of this section about the conservativeness of the TF-QKD key rates plotted in Fig. S3.

# Final considerations

In our security argument, we let Eve play the role of Charlie and she acts as a completely untrusted party. Also, Alice and Bob do not possess measuring devices. The virtual measurements related to the schemes in Figs. S2c-S2f are not really executed by the users and they are merely tools for the security argument. This qualifies TF-QKD as a measurement-device-independent scheme.

To prove security, we assumed that the two transmitters are perfectly locked, similarly to phase-based MDI-QKD.[18] We have then shown that this condition is not restrictive because imperfect phase locking would only introduce a basis-independent noise. However, it seems interesting to discuss how feasible this assumption is in practice.

Experiments on first-order interference of light beams emitted from independent lasers have been performed for 50 years now[17] and it is not difficult to replicate them with good interference visibility. Although the frequency matching between the two independent lasers is more demanding than in second-order interference,[89,90] it can be achieved using optical phase-lock loop (OPLL) techniques.[27,28] These are well-known elements in optical communications and can stabilise the frequency of two distant lasers to less than 1 Hz over 1000 seconds.[29]

In OPLL, the light beams from a master laser and a slave laser interfere on a beam splitter and generate a beating signal.[28] The resulting signal is measured by a photodiode, whose output is amplified, filtered and used to adjust the frequency of the slave laser. Security-wise, it is important to note that the cavities of the two lasers are not in optical contact. This entails a higher practical security than attained, e.g., using laser seeding,[91] where the cavities of the lasers are in direct contact.

We expect that other limitations of the scheme, related to an asymmetric implementation of TF-QKD, will not spoil the overall performance. For instance, an intensity mismatch on Charlie's beam splitter would not affect the interference visibility considerably. If $\delta I$ represents the intensity fluctuation and $I$ the average intensity, the visibility scales at worst linearly with $\delta I/I$. The contribution of a laser source to this ratio is usually very small, even in commercial lasers. On the other hand, the contribution to this ratio from the optical fibre interferometer is modest too, as proven by the 99.65% visibility reported in Fig. 3c. Moreover, the average intensity of each user's laser can be effectively stabilised in time using an optical power meter plus feedback via a variable optical attenuator, as already implemented in QKD systems. Decoy state preparation can be precisely achieved through careful calibration of the intensity modulators. In decoy states, the intensity emitted by the users is only weakly dependent on the channel length, so the users do not have to change their intensity settings if the channels' lengths are not exactly the same. Finally, if the users wanted to match the channel losses, this would be easily realisable with an extra attenuator in Charlie's station.

# Note added after publication

The present paper was published in Ref. [92]. There it was shown that a pair of phase-randomised optical fields, independently and remotely prepared by two users (Alice and Bob), can interfere at a central location (Charlie) and potentially generate cryptographically secure keys from the same principles as QKD.[93] To achieve this, the optical fields should be "twins", i.e., have close enough electromagnetic phases to effectively interfere in Charlie's station. At first sight, this might look intricate, as the phases are first randomised and then reconciled at a later stage. But it is not too different from a Boggle game,[94] where the letters are first scrambled and then recomposed into words to gain points.

If the users correctly and efficiently implement TF-QKD, they will gain some advantages over QKD:

1. The secure key rate of their TF-QKD protocol will scale like $\sqrt{\eta}$, which is similar to the scaling rate of a single-node quantum repeater.[95] Here $\eta$ is the transmittance of the quantum channel between Alice and Bob. This scaling scaling law for a scheme so close to QKD was entirely unknown before the present work. QKD was believed to scale at best linearly with $\eta$.[96,97]

2. Because of the square-root scaling, the key rate of TF-QKD will overcome at long distance the secret key capacity of an uninterrupted quantum channel,[97] as well as the key rate of measurement-device-independent (MDI) QKD[98] (see also [99, 100]), as both scale linearly with $\eta$.

3. The previous points (1) and (2) can be achieved with a scheme
   (a) that is feasible with current technology and is similar to a fibre-based phase-based QKD setup;
   (b) whose security is independent of the measuring devices, as in MDI-QKD.

Let us notice that in the main paper[92] and in point (1) above, we refer to a "quantum repeater" as a physical device specifically designed to store and re-transmit the quantum signals, e.g., through the use of a quantum memory.[101] A single-node quantum repeater is a repeater chain composed by a single intermediate node. In a quantum information-theoretic setting, a quantum repeater can generally be intended as *any* intermediate node helping the quantum communication, even a trusted measure-and-prepare QKD station with a replica of Alice's and Bob's modules.[102] In this perspective, the progress entailed by TF-QKD might look marginal, because the theoretical key rate of a channel with a single-node repeater was already known to scale with $\sqrt{\eta}$.

However, from a theoretical perspective, there is a vast difference between an untrusted node linking Alice and Bob, like in TF-QKD, and a trusted measure-and-prepare QKD station. On the other hand, from an experimental point of view, there is an incommensurate difference between a full-fledged quantum repeater and a measuring station that is composed purely by components borrowed from QKD. The difference is all in the feasibility. Despite substantial progress,[103–115] a quantum repeater still is presently a demanding technology. On the contrary, the first QKD experiment was performed almost three decades ago.[116] Since then QKD has steadily progressed, reaching a maturity level suitable for the market. Therefore, it is important to know that the scaling entailed by a single-node quantum repeater can be approached using a QKD-like scheme as simple as TF-QKD. Clearly, TF-QKD does not replace a full-fledged quantum repeater, because it only works with one central node connecting two end users and it cannot be concatenated in order to replace a whole repeater chain.

As a second remark, we should clarify the conditions for the claims (1)-(3) in the above list.

Claims 3(a) and 3(b) are immediate. The proposed TF-QKD scheme[92] is MDI by design. As it can be noted from Fig. 1(b) in,[92] all the measuring devices are outside the secure perimeters of the users and the third party, Charlie, is entirely untrusted. Moreover, it is apparent that the components are the same as in QKD.

Claims (1) and (2) were initially proven in [92] under some restrictive assumptions on the eavesdropper (Eve). These assumptions were clearly stated in Ref. [92], to avoid any misunderstanding. Therefore, we believe that these claims are perfectly legitimate, because the conditions under which they were obtained were clearly pointed out in the paper. The only relevant discussion in this case is about the assumptions, i.e., whether they are too strong or weak enough to guarantee the meaningfulness of the results.

In the development of a new protocol, it is customary and generally well accepted that the initial assumptions are quite strong. Later on, the assumptions are gradually weakened until their complete removal, in the best case. We started by assuming the security of TF-QKD and noticing that it made the detection rate scale favourably. Then we proved that the main features of TF-QKD are not lost if one gets rid of all the assumptions but one, i.e., that the phase announcement does not affect the security of the protocol. This is our main assumption in Ref. [92]. We called it "assumption $A^{(\neg\rho)}$", with reference to not-having information leakage from the announcement of the global phase $\rho$. The TF-QKD key rate equation, Eq. (3) in [92], has been drawn from there.

Afterwards, we partially relaxed this assumption by considering the so-called "collective-beam-splitting" (CBS) attack,[117] described in this Supplementary Information of [92], thus warning the reader, again,

about the presence and the importance of this assumption in TF-QKD. Recently, a more powerful attack leveraging on the $A^{(\neg\rho)}$ assumption has been proposed by X.-B. Wang et al.[118] Although this attack can be mitigated when all the conditions in the original TF-QKD scheme are taken into account,[119] it still highlighted the central role of the $A^{(\neg\rho)}$ assumption and the necessity to drop it and develop unconditional security proofs for TF-QKD.

Fortunately, we have witnessed a quick progress in this direction with several security proofs of TF-QKD-like protocols[123–128] that do not rely on the $A^{(\neg\rho)}$ assumption, nor on other limiting assumptions for the eavesdropper. This ultimately proves the correctness of the initial idea and paves the way to further progress in this field.

# References


[31] H. Takesue, S. W. Nam, Q. Zhang, R. H. Hadfield, T. Honjo, K. Tamaki, & Y. Yamamoto. Quantum key distribution over a 40-db channel loss using superconducting single-photon detectors. *Nat. Photon.* **1**, 343 (2007).

[32] D. Rosenberg, C. G. Peterson, J. W. Harrington, P. R. Rice, N. Dallmann, K. T. Tyagi, K. P. McCabe, S. Nam, B. Baek, R. H. Hadfield, R. J. Hughes, & J. E. Nordholt. Practical long-distance quantum key distribution system using decoy levels. *New J. Phys.* **11**, 045009 (2009).

[33] D. Stucki, N. Gisin, O. Guinnard, G. Ribordy, & H. Zbinden. High rate, long-distance quantum key distribution over 250 km of ultra low loss fibres. *New J. Phys.* **11**, 075003 (2009).

[34] Z. L. Yuan, A. R. Dixon, J. F. Dynes, A. W. Sharpe & A. J. Shields. Practical gigahertz quantum key distribution based on avalanche photodiodes. *New J. Phys.* **11**, 045019 (2009).

[35] Y. Liu, T.-Y. Chen, J. Wang, W.-Q. Cai, X. Wan, L.-K. Chen, J.-H. Wang, S.-B. Liu, H. Liang, L. Yang, C.-Z. Peng, K. Chen, Z.-B. Chen, & J.-W. Pan. Decoy-state quantum key distribution with polarized photons over 200 km. *Opt. Express* **18**, 8587 (2010).

[36] N. Namekata, H. Takesue, T. Honjo, Y. Tokura & S. Inoue. High-rate quantum key distribution over 100 km using ultra-low-noise, 2-GHz sinusoidally gated InGaAs/InP avalanche photodiodes. *Opt. Express* **19**, 10632 (2011).

[37] S. Wang, W. Chen, J.-F. Guo, Z.-Q. Yin, H.-W. Li, Z. Zhou, G.-C. Guo, & Z.-F. Han. 2 GHz clock quantum key distribution over 260 km of standard telecom fiber. *Opt. Lett.* **37**, 1008 (2012).

[38] P. Jouguet, S. Kunz-Jacques, A. Leverrier, P. Grangier, & E. Diamanti. Experimental demonstration of long-distance continuous-variable quantum key distribution. *Nat. Photon.* **7**, 378 (2013).

[39] K. Shimizu, T. Honjo, M. Fujiwara, T. Ito, K. Tamaki, S. Miki, T. Yamashita, H. Terai, Z. Wang, & M. Sasaki. Performance of long-distance quantum key distribution over 90-km optical links installed in a field environment of Tokyo metropolitan area. *J. Lightwave Technol.* **32**, 141 (2014).

[40] B. Korzh, C. C. W. Lim, R. Houlmann, N. Gisin, M. J. Li, D. Nolan, B. Sanguinetti, R. Thew, & H. Zbinden. Provably secure and practical quantum key distribution over 307 km of optical fibre. *Nat. Photon.* **9**, 163 (2015).

[41] D. Huang, D. Lin, C. Wang, W. Liu, S. Fang, J. Peng, P. Huang, & G. Zeng. Continuous-variable quantum key distribution with 1 Mbps secure key rate. *Opt. Expr.* **23**, 17511 (2015).

[42] L. C. Comandar, M. Lucamarini, B. Fröhlich, J. F. Dynes, A. W. Sharpe, S. W.-B. Tam, Z. L. Yuan, R. V. Penty, & A. J. Shields. Quantum key distribution without detector vulnerabilities using optically seeded lasers. *Nat. Photon.* **10**, 312 (2016).

[43] D. Huang, P. Huang, D. Lin & G. Zeng. Long-distance continuous-variable quantum key distribution by controlling excess noise. *Sci. Rep.* **6**, 19201 (2016).

[44] B. Fröhlich, M. Lucamarini, J. F. Dynes, L. C. Comandar, W. W.-S. Tam, A. Plews, A. W. Sharpe, Z. Yuan, & A. J. Shields. Long-distance quantum key distribution secure against coherent attacks. *Optica* **4**, 163 (2017).

[45] S. Pirandola, R. García-Patrón, S. L. Braunstein & S. Lloyd. Direct and reverse secret-key capacities of a quantum channel. *Phys. Rev. Lett.* **102**, 050503 (2009).

[46] M. M. Wilde, M. Tomamichel & M. Berta. Converse bounds for private communication over quantum channels. *IEEE Trans. Inf. Theory* **63**, 1792-1817 (2017).
[47] P. W. Shor & J. Preskill. Simple proof of security of the BB84 quantum key distribution protocol. *Phys. Rev. Lett.* **85**, 441 (2000).
[48] F. Xu, M. Curty, B. Qi & H.-K. Lo. Practical aspects of measurement-device-independent quantum key distribution. *New J. Phys.* **15**, 113007 (2013).
[49] X. Ma, B. Qi, Y. Zhao & H.-K. Lo. Practical decoy state for quantum key distribution. *Phys. Rev. A* **72**, 012326 (2005).
[50] M. Koashi. Efficient quantum key distribution with practical sources and detectors. Preprint at https://arxiv.org/abs/quant-ph/0609180 (2006).
[51] K. Tamaki, M. Curty & M. Lucamarini. Decoy-state quantum key distribution with a leaky source. *New J. Phys.* **18**, 065008 (2016).
[52] K. Tamaki, M. Curty, G. Kato, H.-K. Lo & K. Azuma. Loss-tolerant quantum cryptography with imperfect sources. *Phys. Rev. A* **90**, 052314 (2014).
[53] A. Ferenczi, V. Narasimhachar & N. Lütkenhaus. Security proof of the unbalanced phase-encoded BB84 protocol. *Phys. Rev. A* **86**, 042327 (2012).
[54] H.-W. Li, Z.-Q. Yin, Z.-F. Han, W.-S. Bao, G.-C. Guo. Security of practical phase-coding quantum key distribution. *Quant. Inf. Comp.* **10**, 0771 (2010).
[55] S. Sunohara, K. Tamaki & N. Imoto. Blind post-processing for the unbalanced BB84. Preprint at https://arxiv.org/abs/1302.1701 (2013).
[56] H.-K. Lo & H. F. Chau. Unconditional security of quantum key distribution over arbitrarily long distances. *Science* **283**, 2050 (1999).
[57] M. Koashi. Simple security proof of quantum key distribution based on complementarity. *New J. Phys.* **11**, 045018 (2009).
[58] A. R. Calderbank & P. Shor. Good quantum error-correcting codes exist. *Phys. Rev. A* **54**, 1098 (1996).
[59] A. M. Steane. Multiple-particle interference and quantum error correction. *Proc. R. Soc. London A* **452**, 2551 (1996).
[60] C. H. Bennett, D. P. DiVincenzo, J. A. Smolin & W. K. Wootters. Mixed-state entanglement and quantum error correction. *Phys. Rev. A* **54**, 3824 (1996).
[61] G. Brassard & L. Salvail. Secret-key reconciliation by public discussion. *Advances in Cryptology – EUROCRYPT '93* , 410-423 (1994).
[62] R. G. Gallager. Low density parity check codes. *Monograph, M.I.T. Press* (1963).
[63] C. H. Bennett, G. Brassard & J. Robert. Privacy amplification by public discussion. *SIAM J. Comput.* **17**, 210-229 (1988).
[64] C. H. Bennett, G. Brassard, C. Crepeau & U. M. Maurer. Generalized privacy amplification. *IEEE Trans. Inf. Theory* **41**, 1915 (1995).
[65] G. Brassard, N. Lütkenhaus, T. Mor & B. C. Sanders. Limitations on practical quantum cryptography. *Phys. Rev. Lett.* **85**, 1330 (2000).
[66] J. Calsamiglia, S. M. Barnett, & N. Lütkenhaus. Conditional beam-splitting attack on quantum key distribution. *Phys. Rev. A* **65**, 012312 (2001).
[67] D. Kahn. *The codebreakers: The story of secret writing.* New York [Rev. ed.], Scribner (1996). ISBN 0-684-83130-9.
[68] S. Fehr & L. Salvail. Quantum authentication and encryption with key recycling. Preprint at https://arxiv.org/abs/1610.05614 (2016).
[69] Z. Cao, Z. Zhang, H.-K. Lo and X. Ma. Discrete-phase-randomized coherent state source and its application in quantum key distribution. *New J. Phys.* **17**, 053014 (2015).
[70] S. J. van Enk & C. A. Fuchs. Quantum state of a propagating laser field. *Quant. Inf. Comp.* **2**, 151-165 (2002).
[71] H.-K. Lo & J. Preskill. Security of quantum key distribution using weak coherent states with non-random phases. *Quant. Inf. and Comput.* **8**, 431-458 (2007).

[72] H. Inamori, N. Lütkenhaus & D. Mayers. Unconditional security of practical quantum key distribution. *Eur. Phys. J. D* **41**, 599 (2007).
[73] N. J. Beaudry, T. Moroder & N. Lütkenhaus. Squashing models for optical measurements in quantum communication. *Phys. Rev. Lett.* **101**, 093601 (2008).
[74] T. Tsurumaru & K. Tamaki. Security proof for quantum-key-distribution systems with threshold detectors. *Phys. Rev. A* **78**, 032302 (2008).
[75] X. Ma, C.-H. F. Fung, J.-C. Boileau & H. F. Chau. Practical post-processing for quantum-key-distribution experiments. *Comput. Security* **30**, 172 (2011).
[76] M. Heid & N. Lütkenhaus. Efficiency of coherent-state quantum cryptography in the presence of loss: influence of realistic error correction. *Phys. Rev. A* **73**, 052316 (2006).
[77] V. Scarani, H. Bechmann-Pasquinucci, N. J. Cerf, M. Dušek, Norbert Lütkenhaus, & M. Peev. The security of practical quantum key distribution. *Rev. Mod. Phys.* **81**, 1301 (2009).
[78] U. Herzog & J. A. Bergou. Distinguishing mixed quantum states: minimum-error discrimination versus optimum unambiguous discrimination. *Phys. Rev. A* **70**, 022302 (2004).
[79] C. W. Helstrøm. *Quantum Detection and Estimation Theory.* Academic Press, New York (1976).
[80] I. D. Ivanovic. How to differentiate between non-orthogonal states. *Phys. Lett. A* **123**, 257 (1987).
[81] D. Dieks. Overlap and distinguishability of quantum states. *Phys. Lett. A* **126**, 303 (1988).
[82] A. Peres. How to differentiate between non-orthogonal states. *Phys. Lett. A* **128**, 19 (1988).
[83] A. S. Holevo. Bounds for the quantity of information transmitted by a quantum communication channel. *Probl. Inf. Transm.* **9**, 177 (1973).
[84] I. Devetak & A. Winter. Distillation of secret key and entanglement from quantum states. *Proc. R. Soc. London, Ser. A* **461**, 207 (2005).
[85] http://www.scontel.ru/products/sspd.
[86] V. A. Seleznev, A. V. Divochiy, Y. B. Vakhtomin, P. V. Morozov, P. I. Zolotov, D. D. Vasil'ev, K. M. Moiseev, E. I. Malevannaya, & K. V. Smirnov. Superconducting detector of IR single-photons based on thin WSi films. *Journal of Physics: Conference Series* **737**, 012032 (2016).
[87] M. A. Nielsen & I. L. Chuang. *Quantum computation and quantum information.* Cambridge University Press, New York, NY, USA (2000).
[88] S. M. Barnett. *Quantum information.* Oxford University Press, Oxford (2009).
[89] Z. L. Yuan, M. Lucamarini, J. F. Dynes, B. Fröhlich, M. B. Ward, & A. J. Shields. Interference of short optical pulses from independent gain-switched laser diodes for quantum secure communications. *Phys. Rev. Appl.* **2**, 064006 (2014).
[90] L. C. Comandar, M. Lucamarini, B. Fröhlich, J. F. Dynes, Z. L. Yuan, & A. J. Shields. Near perfect mode overlap between independently seeded, gain-switched lasers. *Opt. Express* **24**, 17849 (2016).
[91] S.-H. Sun, F. Xu, M.-S. Jiang, X.-C. Ma, H.-K. Lo, and L.-M. Liang. Effect of source tampering in the security of quantum cryptography. *Phys. Rev. A* **92**, 022304 (2015).
[92] M. Lucamarini, Z. L. Yuan, J. F. Dynes, and A. J. Shields, Nature **557**, 400-403 (2018).
[93] C. H. Bennett and G. Brassard, Theor. Comput. Sci. **560**, 7 (2014).
[94] https://en.wikipedia.org/wiki/Boggle.
[95] S. Pirandola, preprint at
https://arxiv.org/abs/1601.00966 (2016).
[96] M. Takeoka, S. Guha, and M. M. Wilde, Nature Commun. **5**, 5235 (2014).
[97] S. Pirandola, R. Laurenza, C. Ottaviani, and L. Banchi, Nature Commun. **8**, 15043 (2017).
[98] H.-K. Lo, M. Curty, and B. Qi, Phys. Rev. Lett. **108**, 130503 (2012).
[99] S. Braunstein and S. Pirandola, Phys. Rev. Lett. **108**, 130502 (2012).
[100] K. Tamaki, H.-K. Lo, C.-H. F. Fung, and B. Qi, Phys. Rev. A **85**, 042307 (2012).
[101] H.-J. Briegel, W. Dür, J. I. Cirac, and P. Zoller, Phys. Rev. Lett. **81**, 5932–5935 (1998).
[102] S. Pirandola, private communication.
[103] T. D. Ladd, P. van Loock, K. Nemoto, W. J. Munro, and Y. Yamamoto, New J. Phys. **8**, 184 (2006).
[104] P. van Loock, T. D. Ladd, K. Sanaka, F. Yamaguchi, K. Nemoto, W. J. Munro, and Y. Yamamoto, Phys. Rev. Lett. **96**, 240501 (2006).

[105] L. Childress, J. M. Taylor, A. S. Sørensen, and M. D. Lukin, Phys. Rev. Lett. **96**, 070504 (2006).
[106] L. Hartmann, B. Kraus, H.-J. Briegel, and W. Dür, Phys. Rev. A **75**, 032310 (2007).
[107] L. Jiang, J. M. Taylor, N. Khaneja, and M. D. Lukin, Proc. Natl. Acad. Sci. U.S.A. **104**, 17291 (2007).
[108] O. A. Collins, S. D. Jenkins, A. Kuzmich, and T. A. B. Kennedy, Phys. Rev. Lett. **98**, 060502 (2007).
[109] L. Jiang, J. M. Taylor, K. Nemoto, W. J. Munro, R. Van Meter, and M. D. Lukin, Phys. Rev. A **79**, 032325 (2009).
[110] S. Bratzik, S. Abruzzo, H. Kampermann, and D. Bruß, Phys. Rev. A **87**, 062335 (2013).
[111] M. Zwerger, H. J. Briegel, and W. Dür, Sci. Rep. **4**, 5364 (2014).
[112] S. Muralidharan, J. Kim, N. Lütkenhaus, M. D. Lukin, and L. Jiang, Phys. Rev. Lett. **112**, 250501 (2014).
[113] K. Azuma, K. Tamaki, and H.-K. Lo, Nat. Commun. **6**, 6787 (2015).
[114] F. Ewert, M. Bergmann, and P. van Loock, Phys. Rev. Lett. **117**, 210501 (2016).
[115] M. Zwerger, A. Pirker, V. Dunjko, H. J. Briegel, and W. Dür, Phys. Rev. Lett. **120**, 30503 (2018).
[116] C. H. Bennett, F. Bessette, G. Brassard, L. Salvail, and J. Smolin, J. Cryptol. **5**, 3 (1992).
[117] We thank N. Lütkenhaus and X. Ma for bringing the beam-splitting attack[116] to our attention during discussions related to the BB84 protocol[93]
[118] X.-B. Wang, X.-L. Hu, and Z.-W. Yu, preprint at https://arxiv.org/abs/1805.02272 (6 May 2018).
[119] The attack addresses the key rate in Eq. (2) in [92], taking the limit of $M \to \infty$, with $M$ the number of phase slices used to reconcile the key bit in TF-QKD (see Fig. 1c in [92]). However, the TF-QKD key rate is given in Ref. [92] by Eq. (3), not by Eq. (2). Eq. (3) contains an extra coefficient $d/M$ that multiplies the remaining part of the key rate. When $M \to \infty$, the key rate in Eq. (3) goes to zero, thus entailing the security of TF-QKD. Even letting $M$ be finite, the attack would cause unusual yields ($Y_0 = Y_{n\geq3} = 0$, $Y_1 = \mu$, $Y_2 = 1$; $\mu$ is the photon flux prepared by Alice and Bob) in the communication which could be detected by the users in a complete implementation of decoy states.[120–122]
[120] W.-Y. Hwang, Phys. Rev. Lett. **91**, 057901 (2003).
[121] X.-B. Wang, Phys. Rev. Lett. **94**, 230503 (2005).
[122] H.-K. Lo, X. Ma, and K. Chen, Phys. Rev. Lett. **94**, 230504 (2005).
[123] X. Ma, P. Zeng, and H. Zhou, Phys. Rev. X **8**, 031043 (2018).
[124] J. Lin and N. Lütkenhaus, Phys. Rev. A **98**, 042332 (2018).
[125] K. Tamaki, H.-K. Lo, W. Wang, and M. Lucamarini, preprint at https://arxiv.org/abs/1805.05511 (15 May 2018).
[126] X.-B. Wang, Z.-W. Yu, X.-L. Hu, preprint at https://arxiv.org/abs/1805.09222 (23 May 2018).
[127] C. Cui, Z.-Q. Yin, R. Wang, W. Chen, S. Wang, G.-C. Guo and Z.-F. Han, preprint at https://arxiv.org/abs/1807.02334 (6 July 2018).
[128] M. Curty, K. Azuma and H.-K. Lo, preprint at https://arxiv.org/abs/1807.07667 (19 July 2018).
